# Supplementary material for: Large-Scale Privacy-Preserving Network Embedding against Private Link Inference Attacks
Source: arXiv:2205.14440 source file (2022-05-28)
Supplement: Supplementary file 1 [file appendix.tex]

\appendix

\section{Appendix}

\subsection{Part One}
\label{subsec:tradeoffappendix}
Privacy-utility tradeoff experimental results on Citeseer and PubMed dataset.
\begin{figure*}[t]
	\centering
	\begin{subfigure}[b]{0.23\textwidth}
		\includegraphics[width=\textwidth]{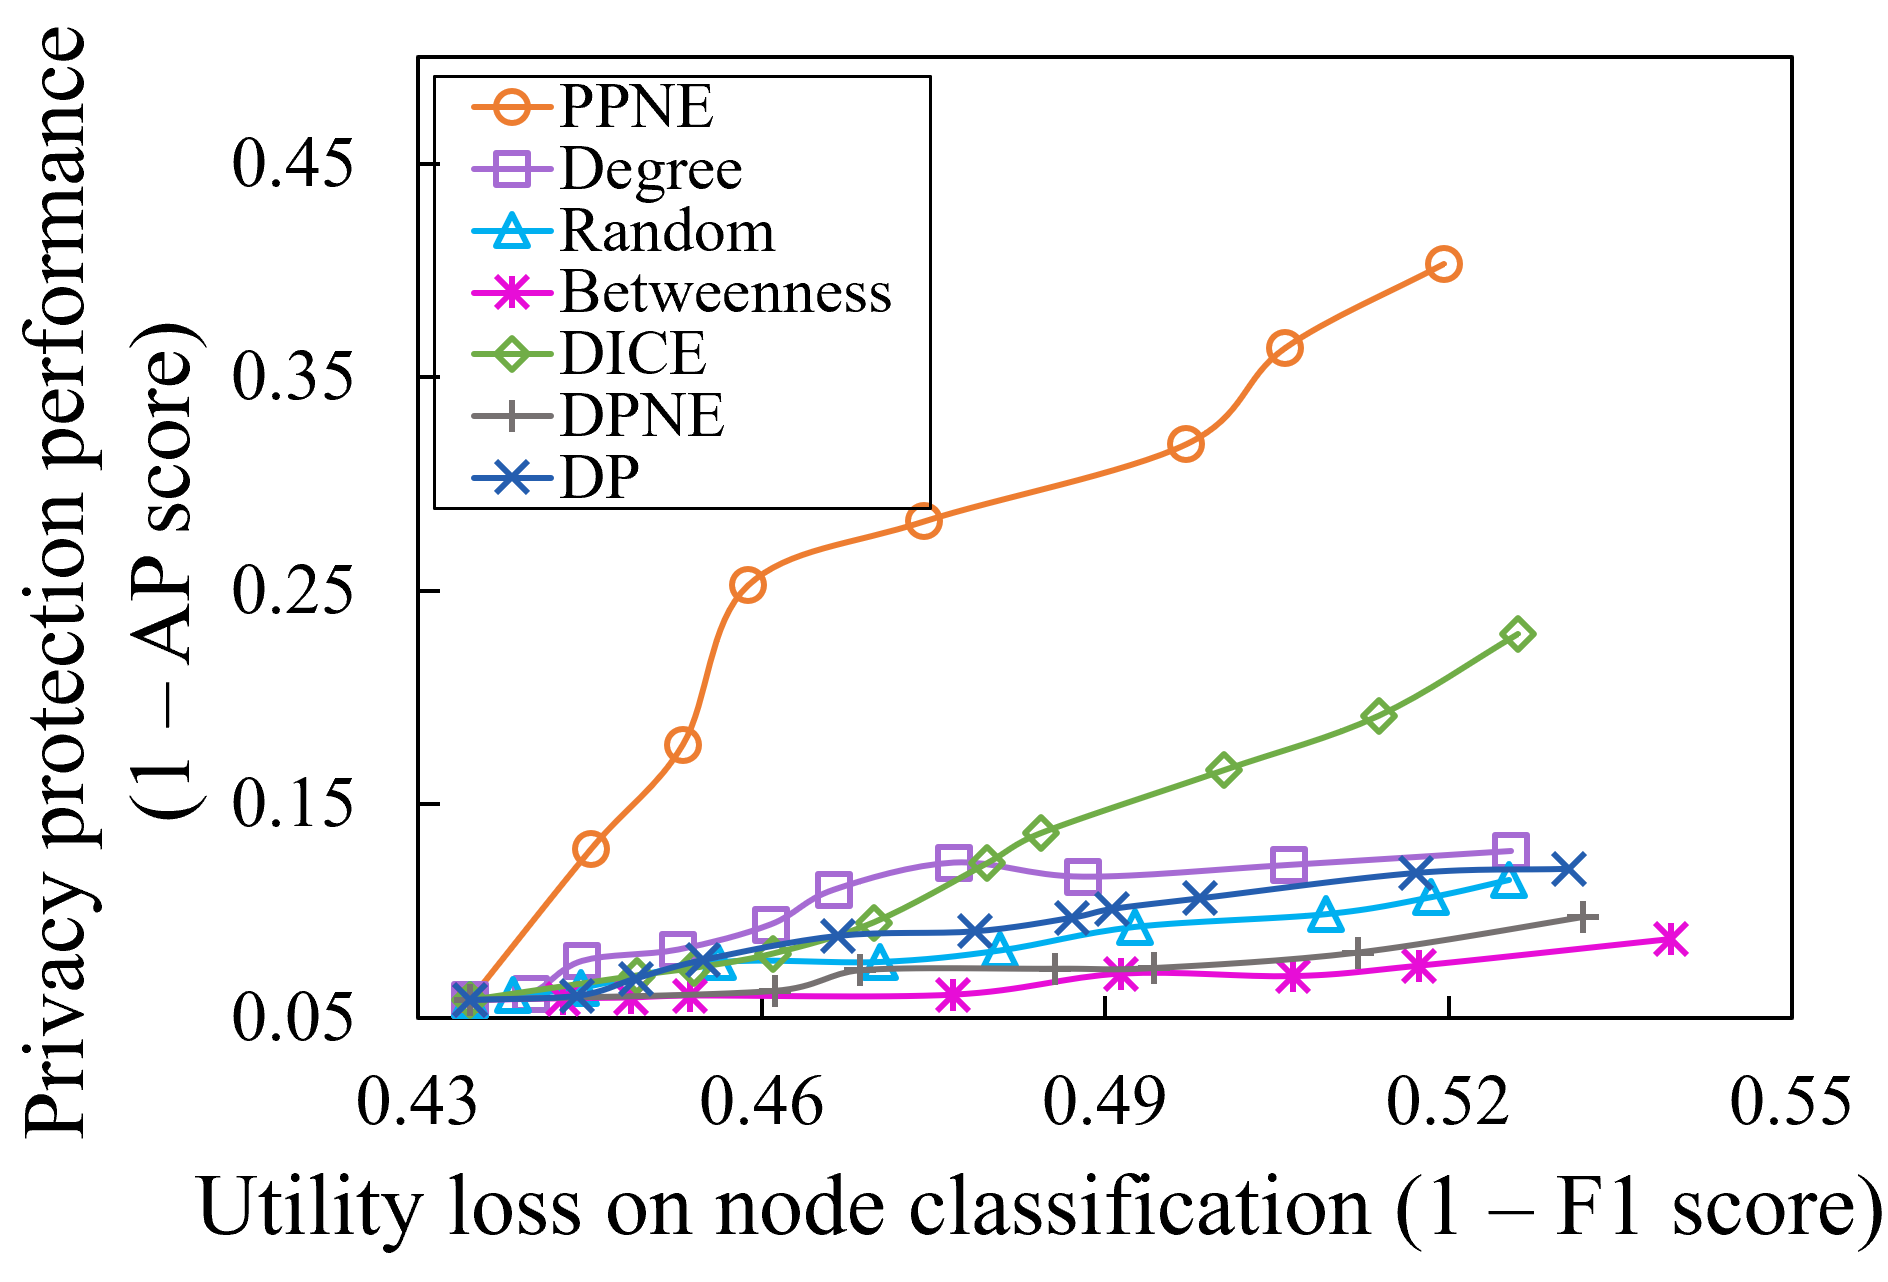}
		\caption{Scenario I on Classification}
		\label{fig:CiteDWSINC}
	\end{subfigure}
	\quad %add desired spacing between images, e. g. ~, \quad, \qquad, \hfill etc.
	%(or a blank line to force the subfigure onto a new line)
	\begin{subfigure}[b]{0.23\textwidth}
		\includegraphics[width=\textwidth]{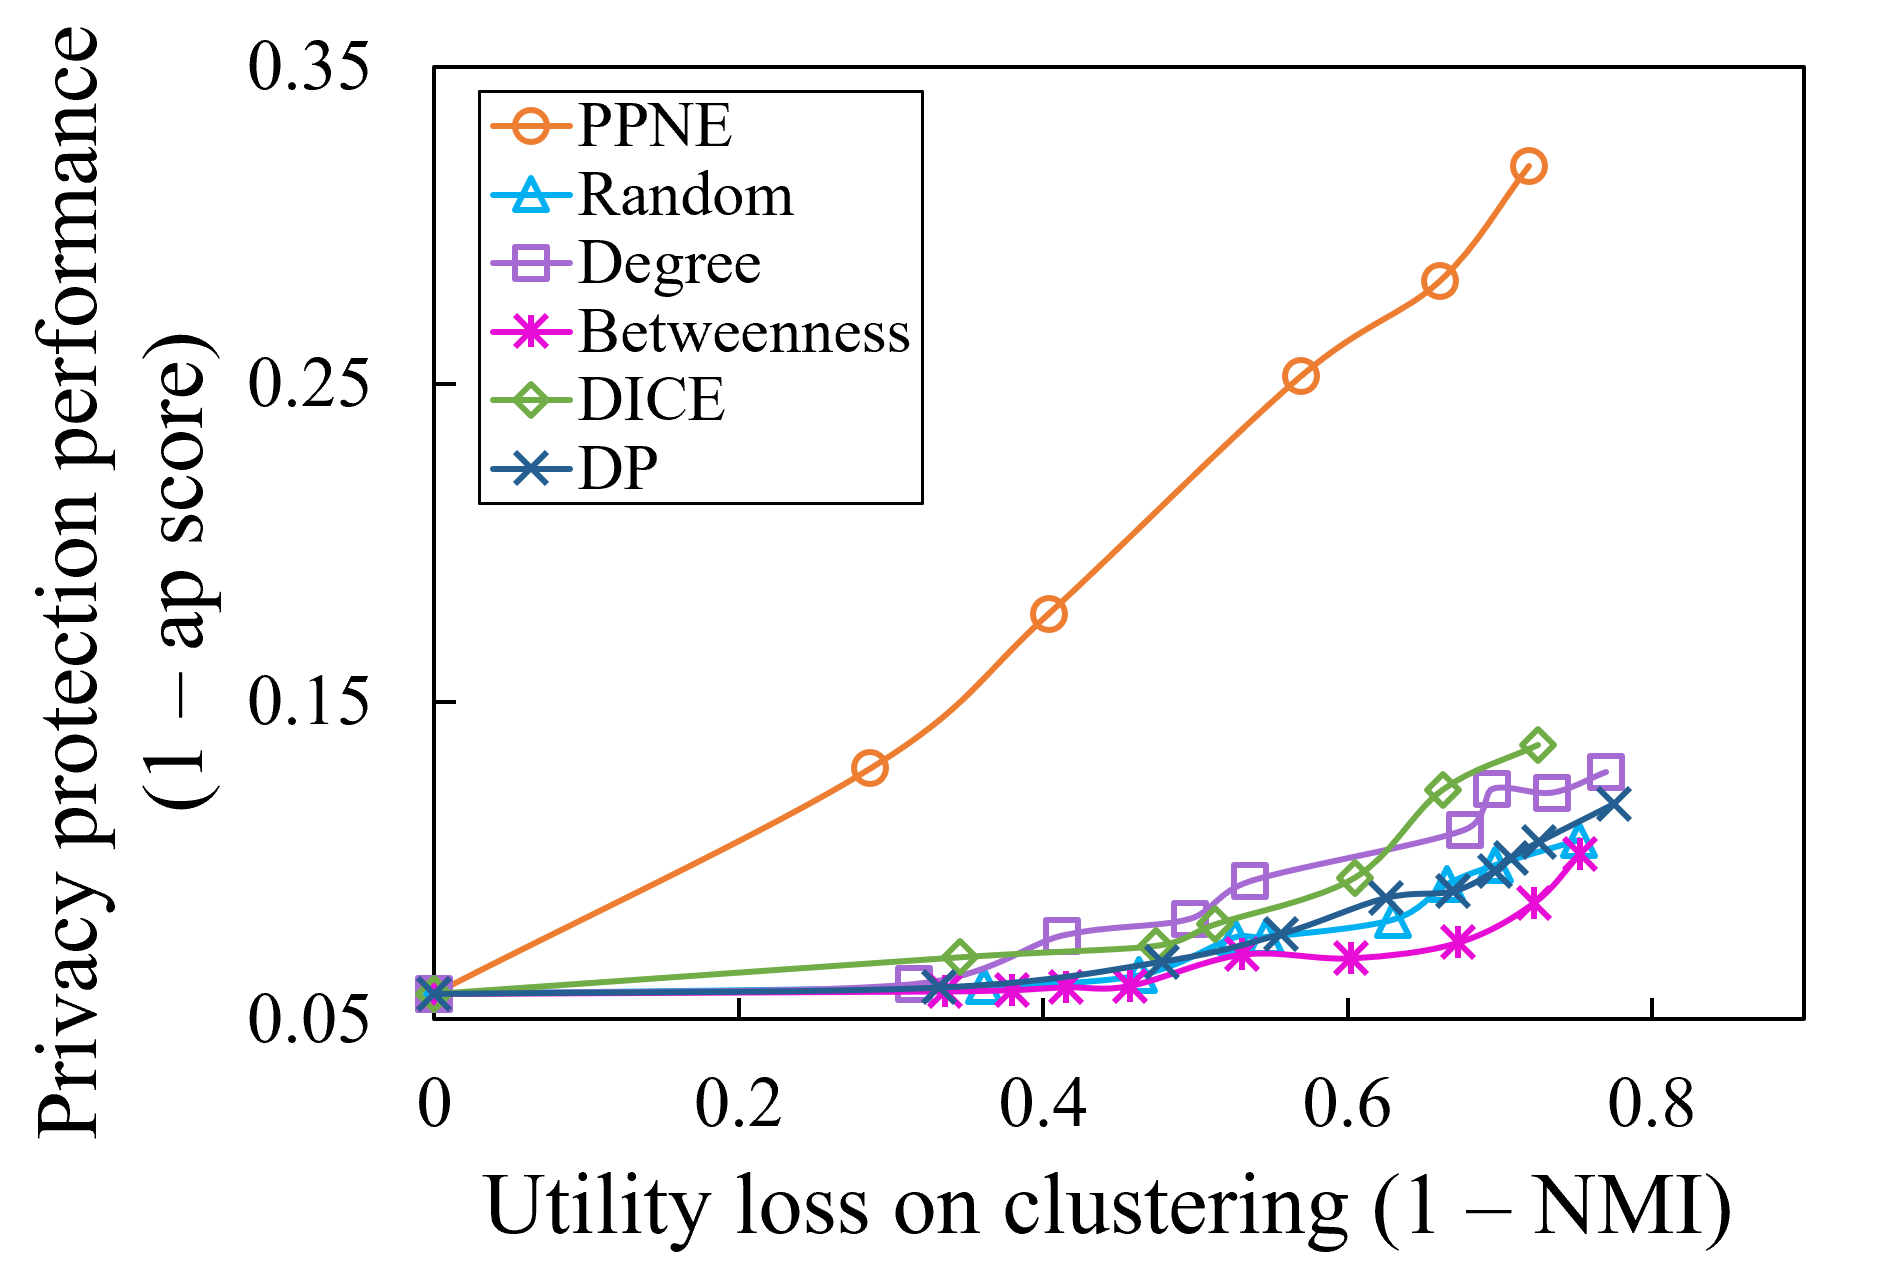}
		\caption{Scenario I on Clustering}
		\label{fig:CiteDWSICL}
	\end{subfigure}
	\quad %add desired spacing between images, e. g. ~, \quad, \qquad, \hfill etc.
	%(or a blank line to force the subfigure onto a new line)
	\begin{subfigure}[b]{0.23\textwidth}
		\includegraphics[width=\textwidth]{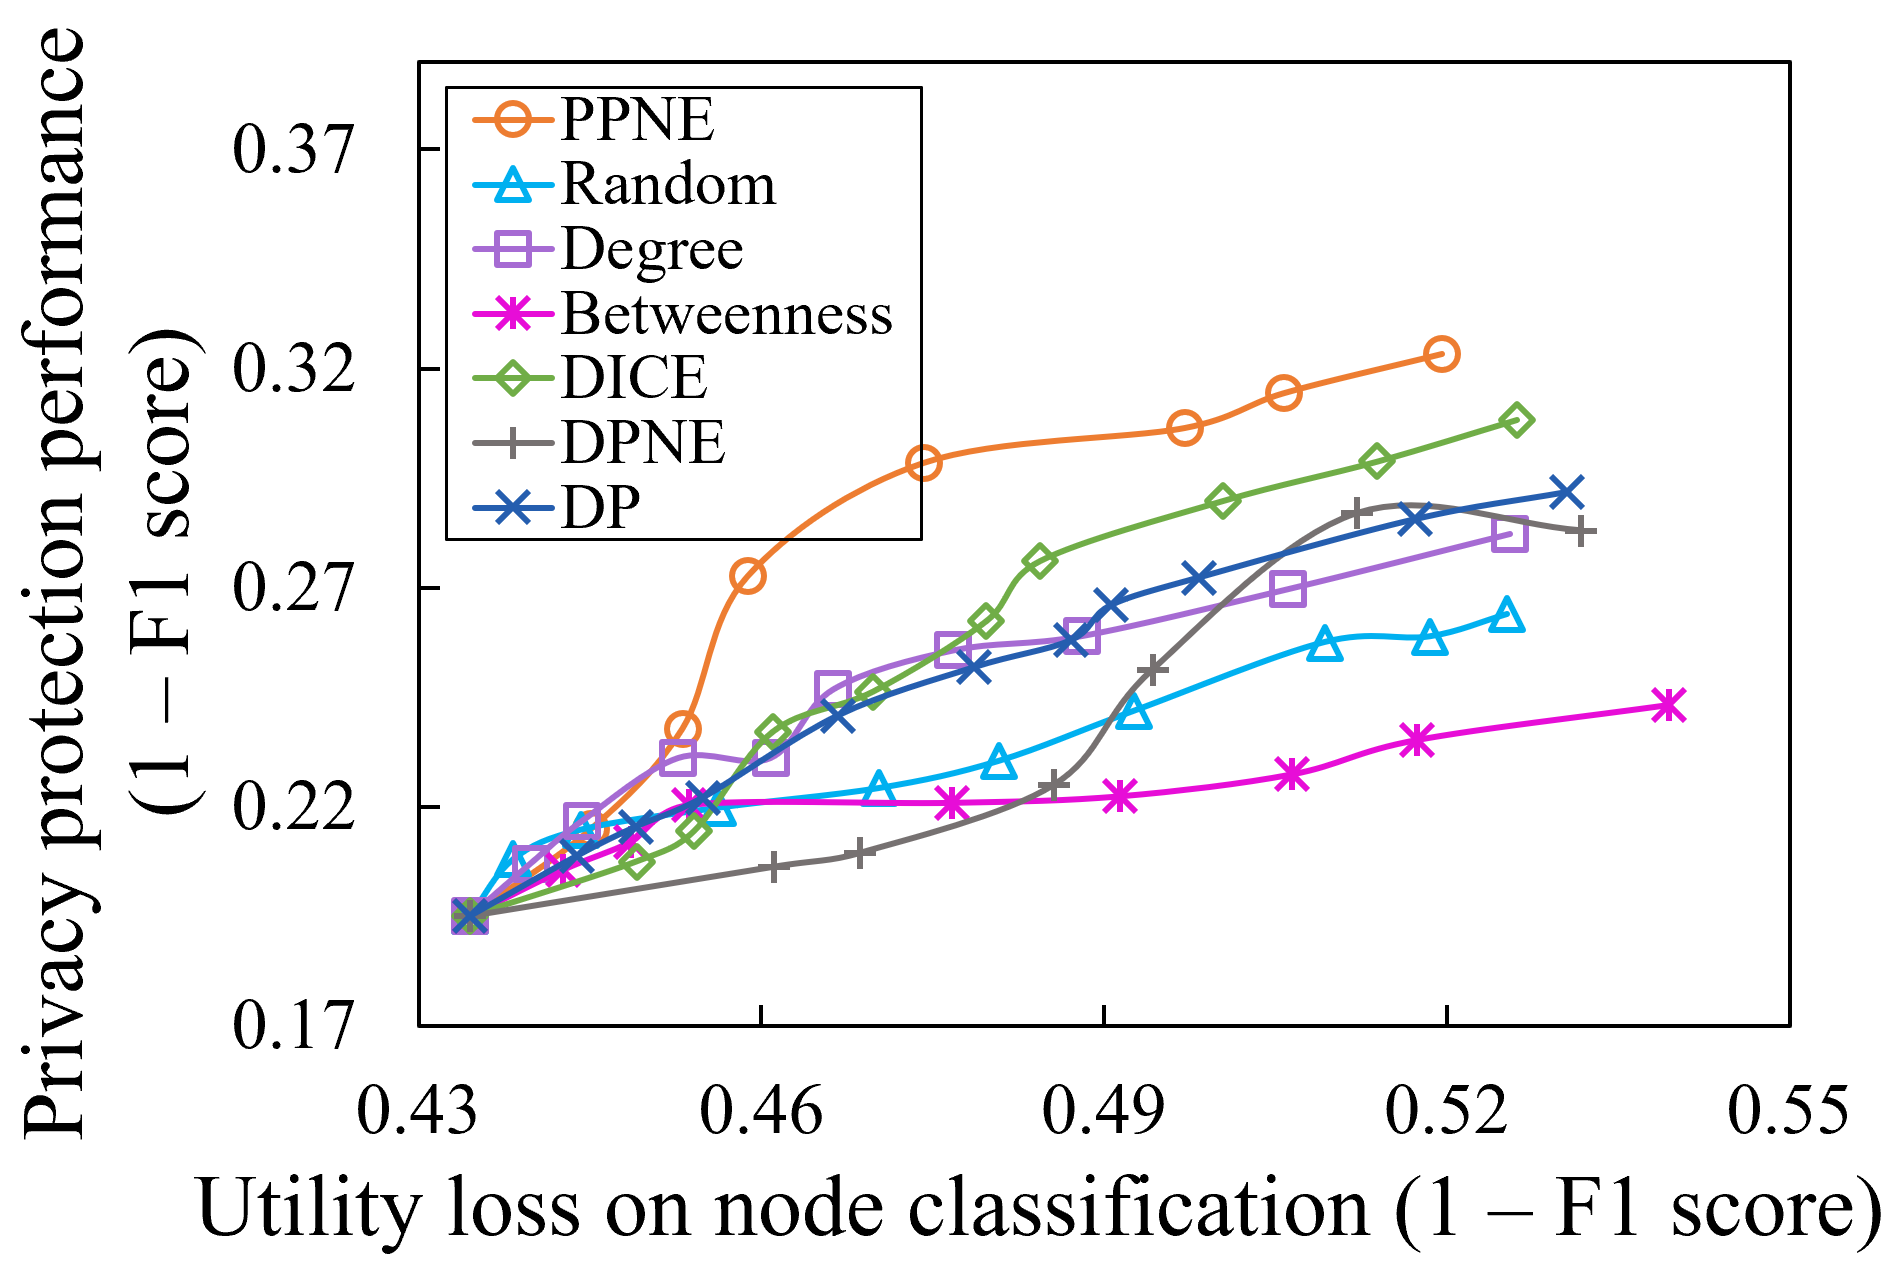}
		\caption{Scenario II on Classification}
		\label{fig:CiteDWSIINC}
	\end{subfigure}
	\quad
	\begin{subfigure}[b]{0.23\textwidth}
		\includegraphics[width=\textwidth]{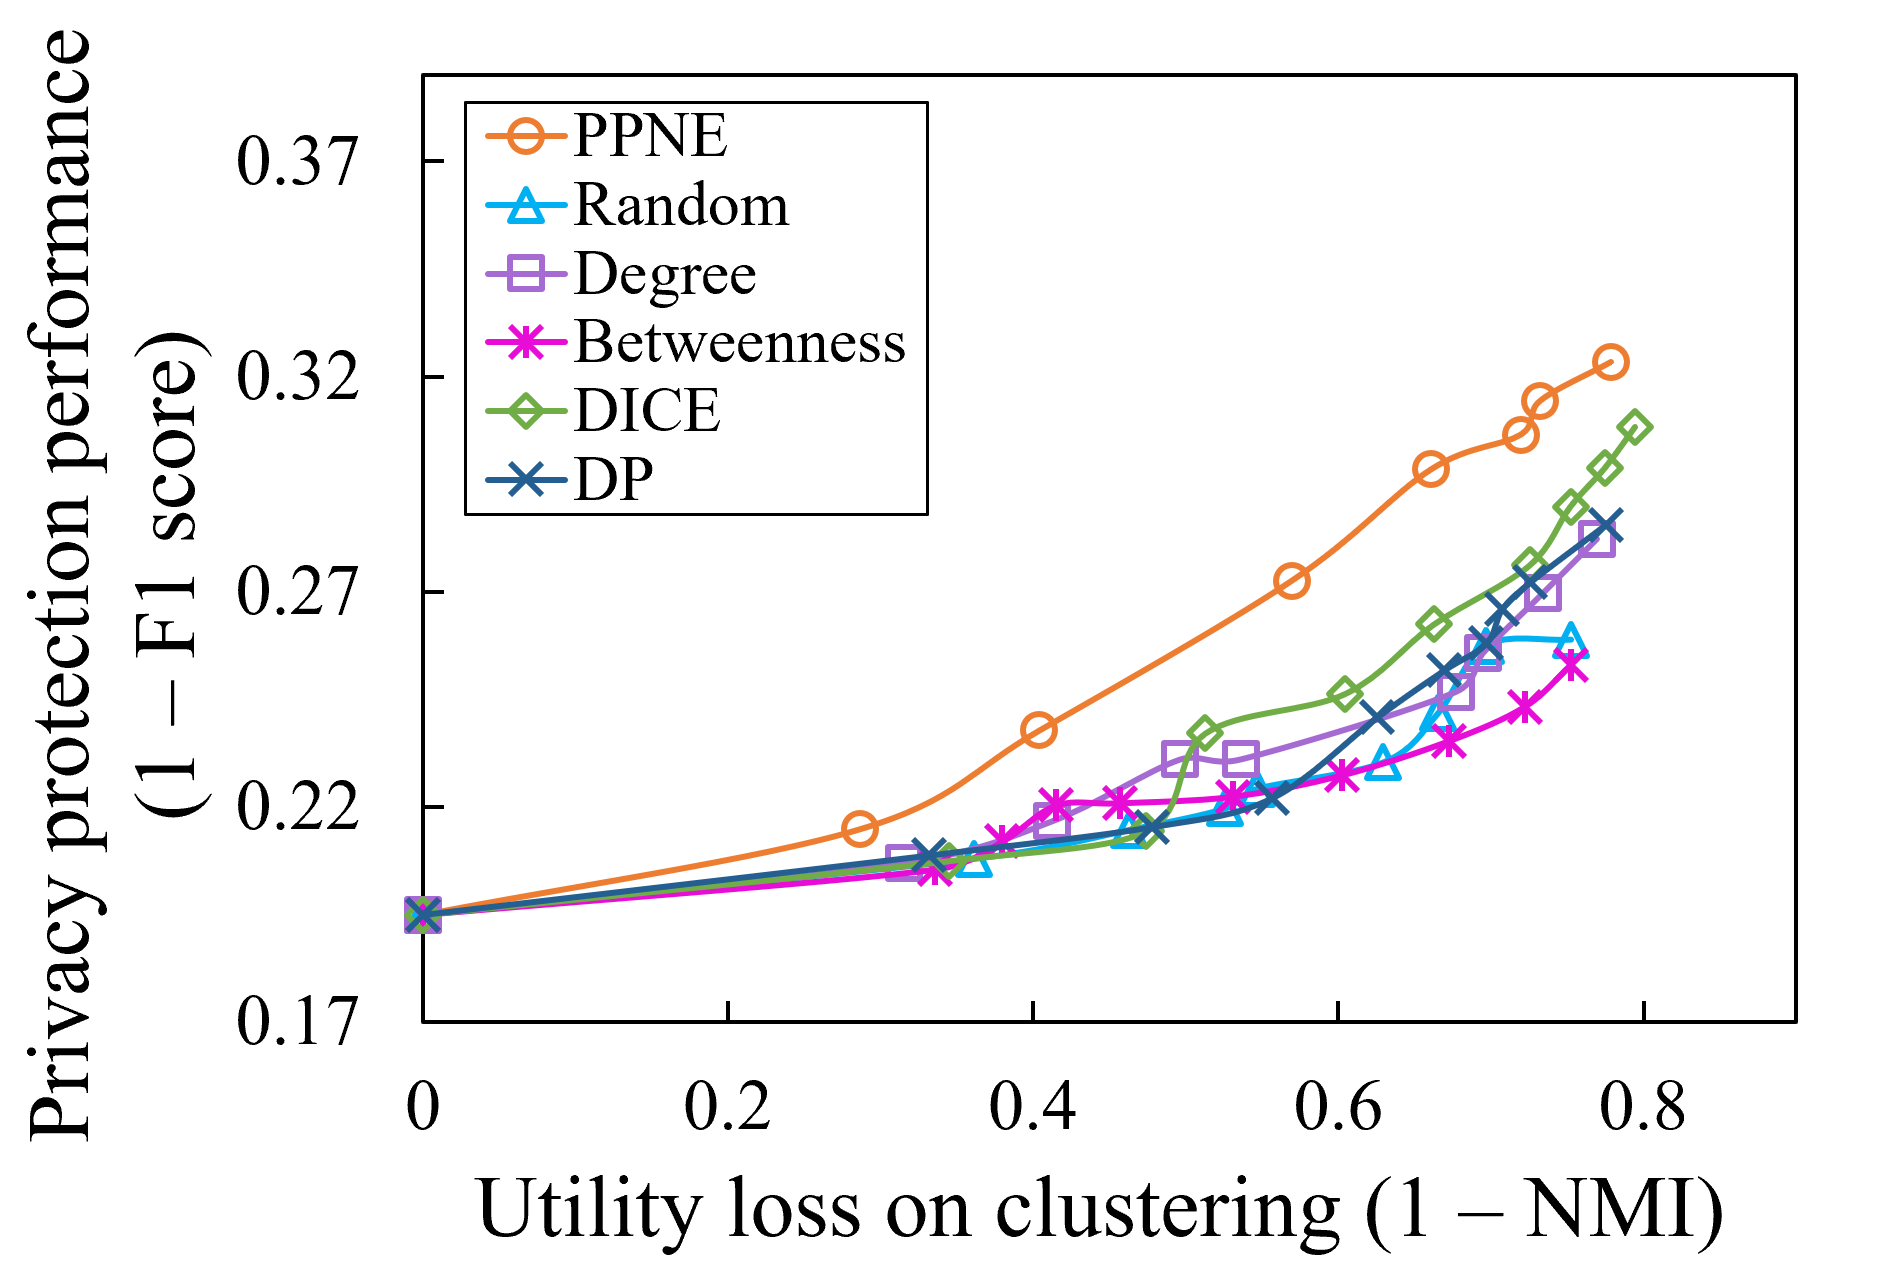}
		\caption{Scenario II on Clustering}
		\label{fig:CiteDWSIICL}
	\end{subfigure}
	\vspace{-1em}
	\caption{Tradeoff on Citeseer: privacy protection on private links and node classification/clustering performance (DeepWalk)}\label{fig:CiteTradeOffDW}
	\vspace{-1em}
\end{figure*}

\begin{figure*}[t]
	\centering
	\begin{subfigure}[b]{0.23\textwidth}
		\includegraphics[width=\textwidth]{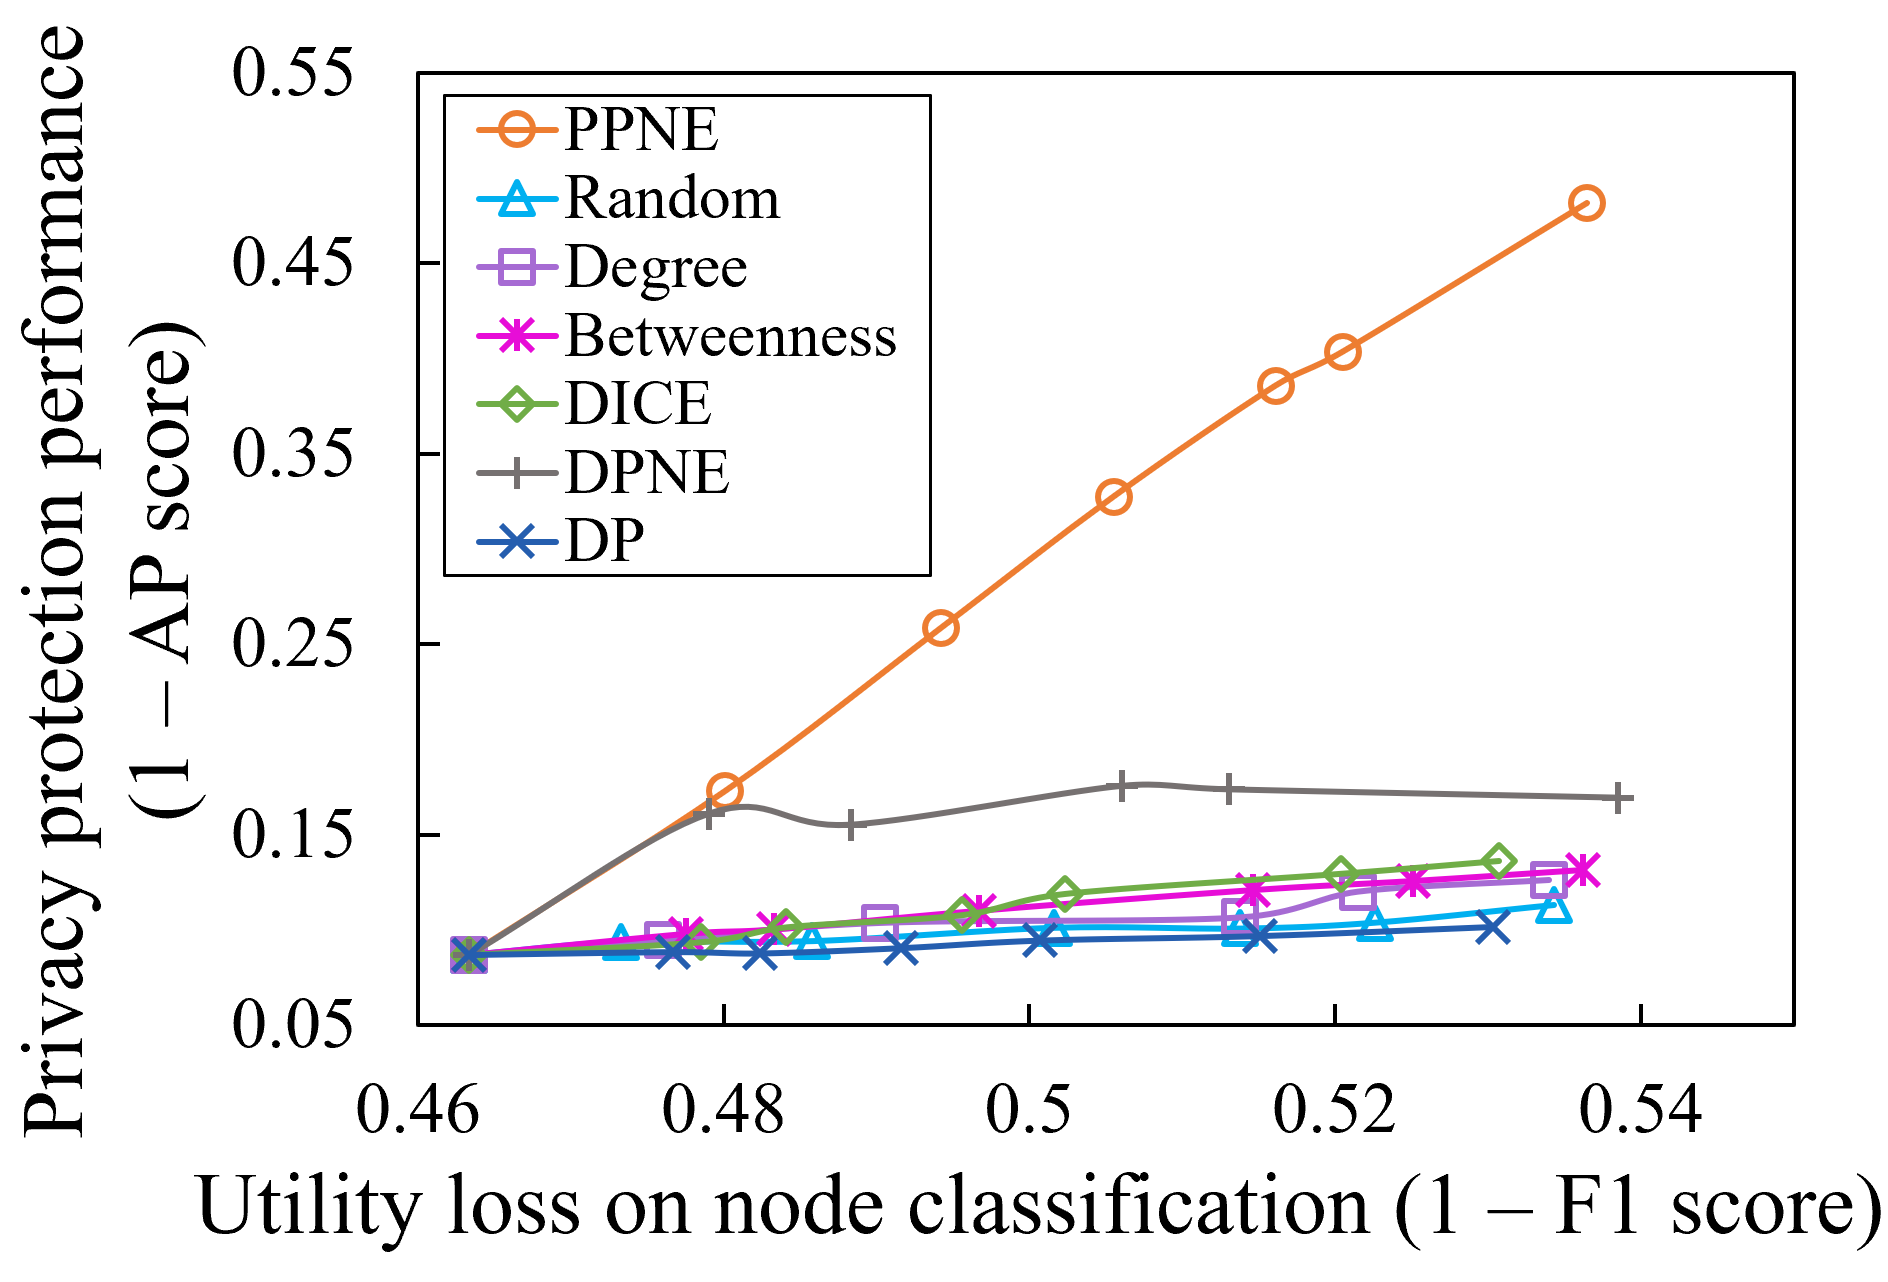}
		\caption{Scenario I on Classification}
		\label{fig:CiteLINESINC}
	\end{subfigure}
	\quad %add desired spacing between images, e. g. ~, \quad, \qquad, \hfill etc.
	%(or a blank line to force the subfigure onto a new line)
	\begin{subfigure}[b]{0.23\textwidth}
		\includegraphics[width=\textwidth]{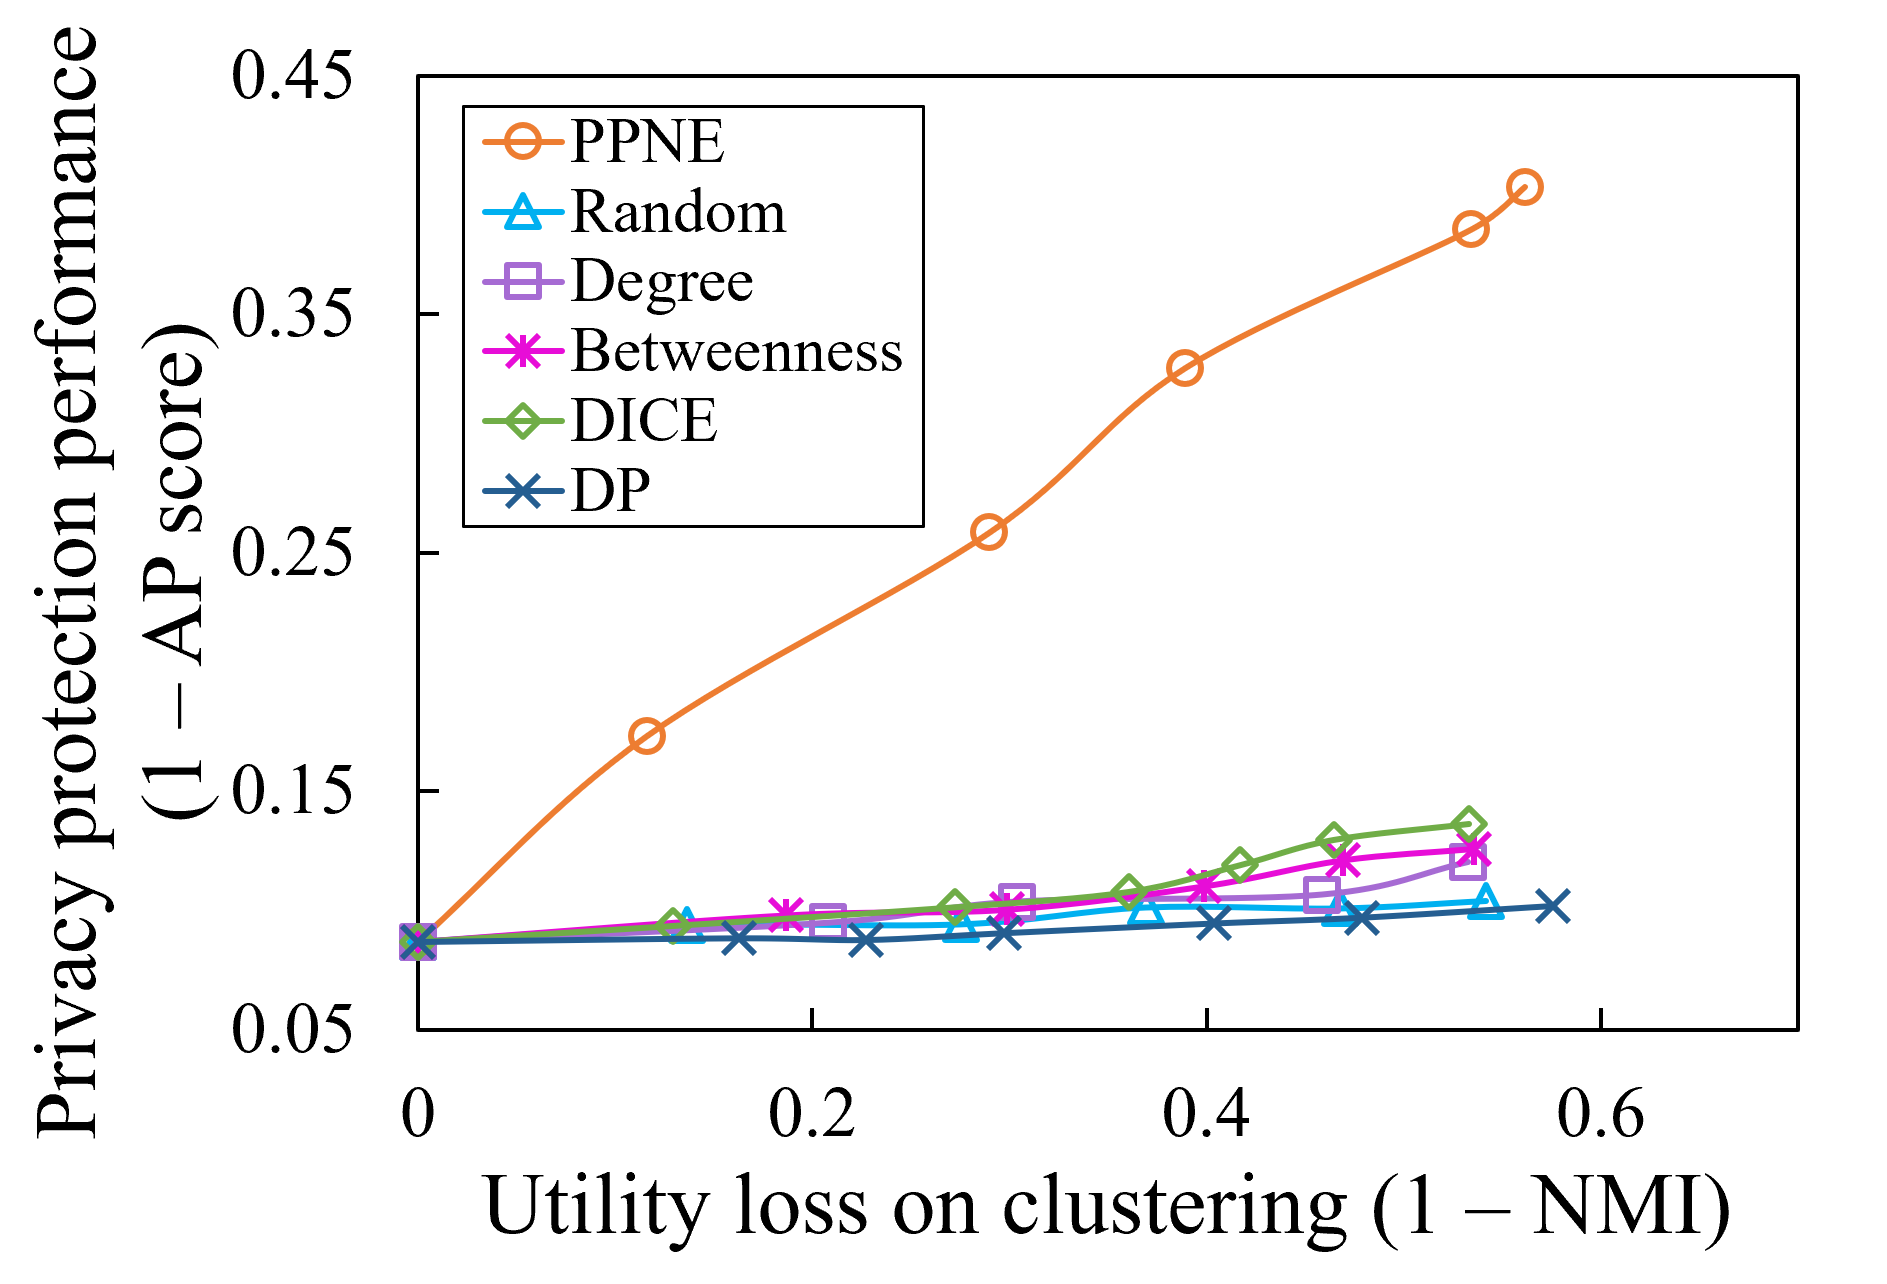}
		\caption{Scenario I on Clustering}
		\label{fig:CiteLINESICL}
	\end{subfigure}
	\quad %add desired spacing between images, e. g. ~, \quad, \qquad, \hfill etc.
	%(or a blank line to force the subfigure onto a new line)
	\begin{subfigure}[b]{0.23\textwidth}
		\includegraphics[width=\textwidth]{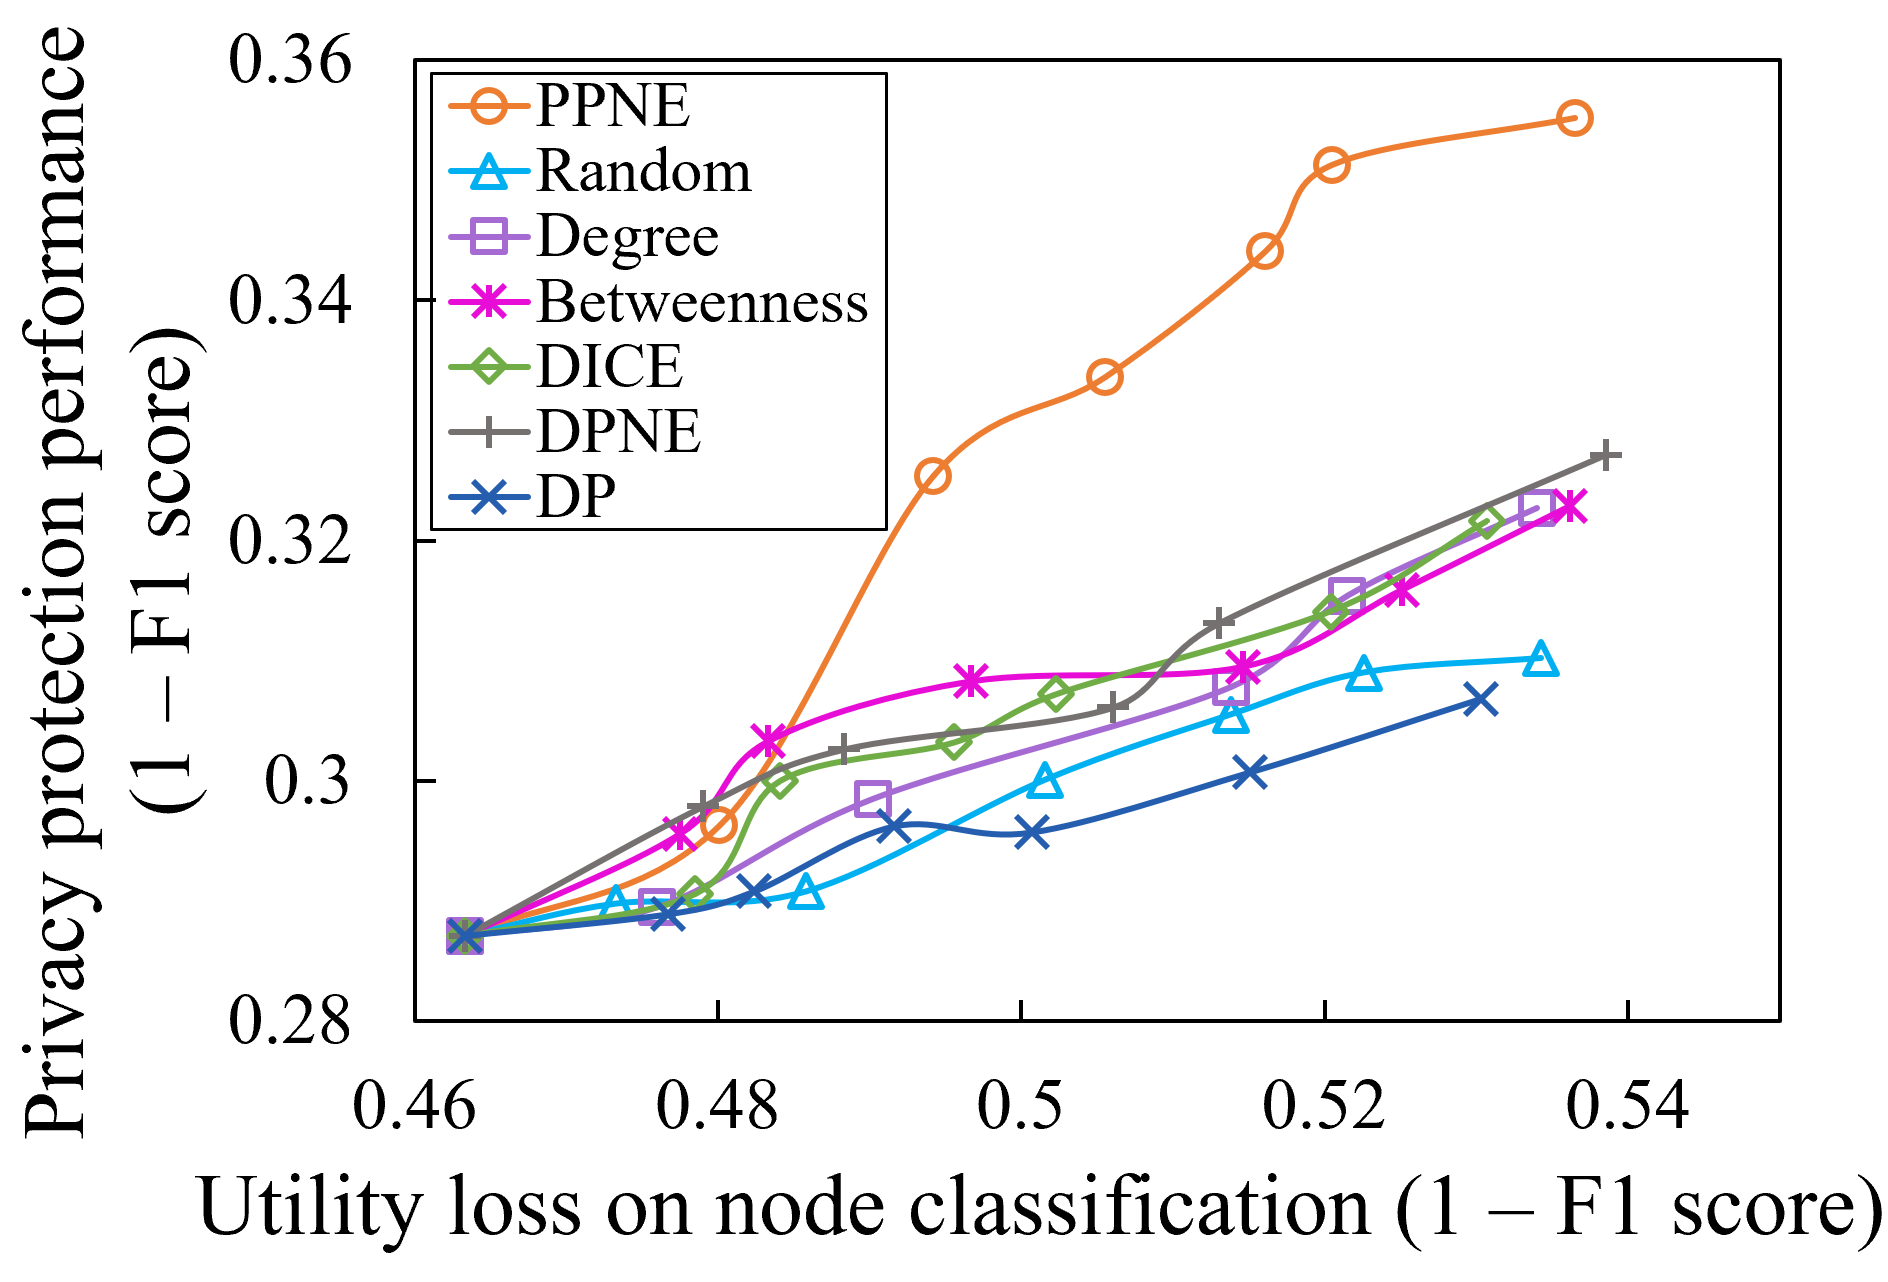}
		\caption{Scenario II on Classification}
		\label{fig:CiteLINESIINC}
	\end{subfigure}
	\quad
	\begin{subfigure}[b]{0.23\textwidth}
		\includegraphics[width=\textwidth]{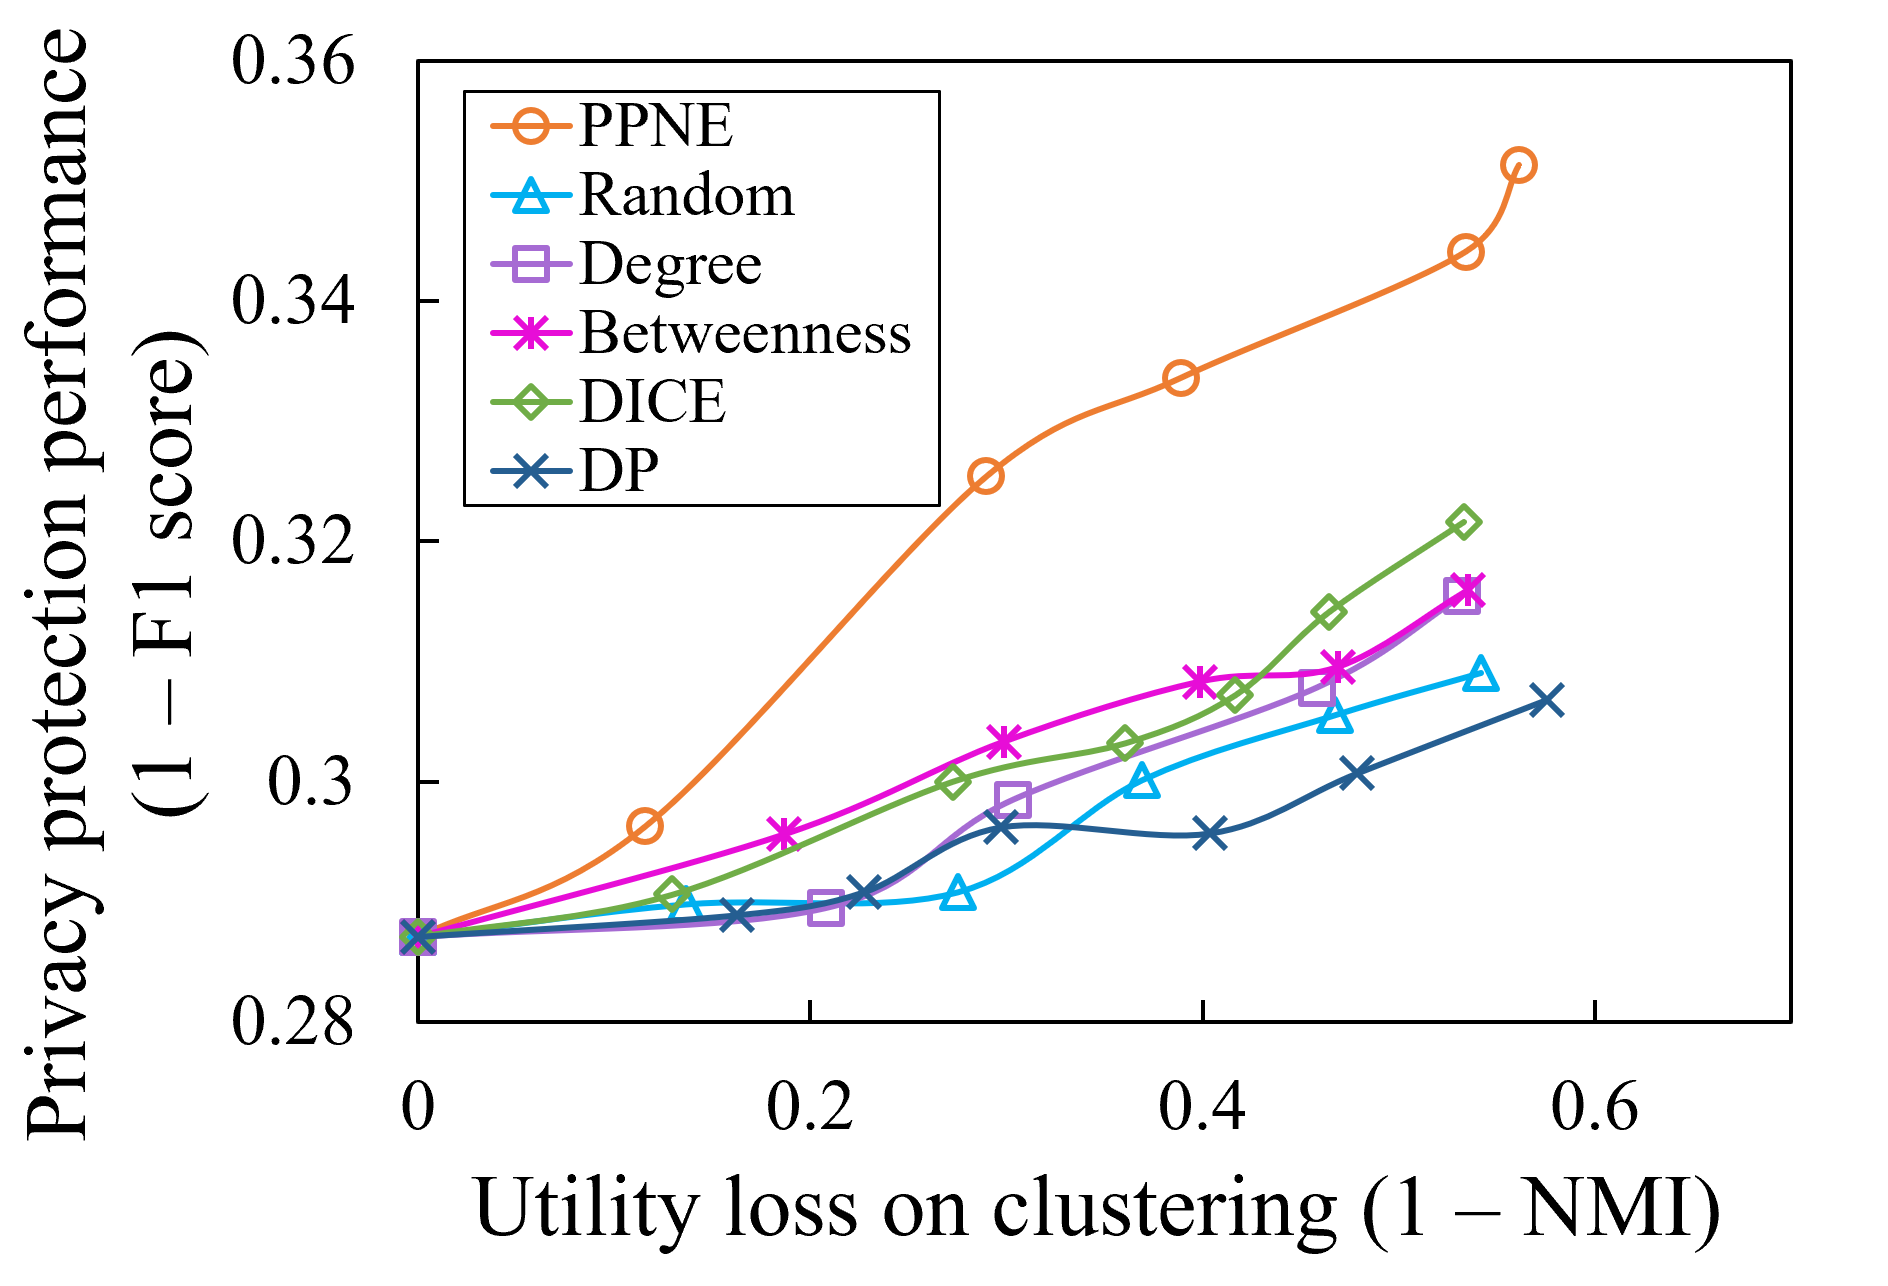}
		\caption{Scenario II on Clustering}
		\label{fig:CiteLINESIICL}
	\end{subfigure}
	\vspace{-1em}
	\caption{Tradeoff on Citeseer: privacy protection on private links and node classification/clustering performance (LINE)}
	\label{fig:CiteTradeOffLINE}
	\vspace{-1em}
\end{figure*}

\begin{figure*}[t]
	\centering
	\begin{subfigure}[b]{0.23\textwidth}
		\includegraphics[width=\textwidth]{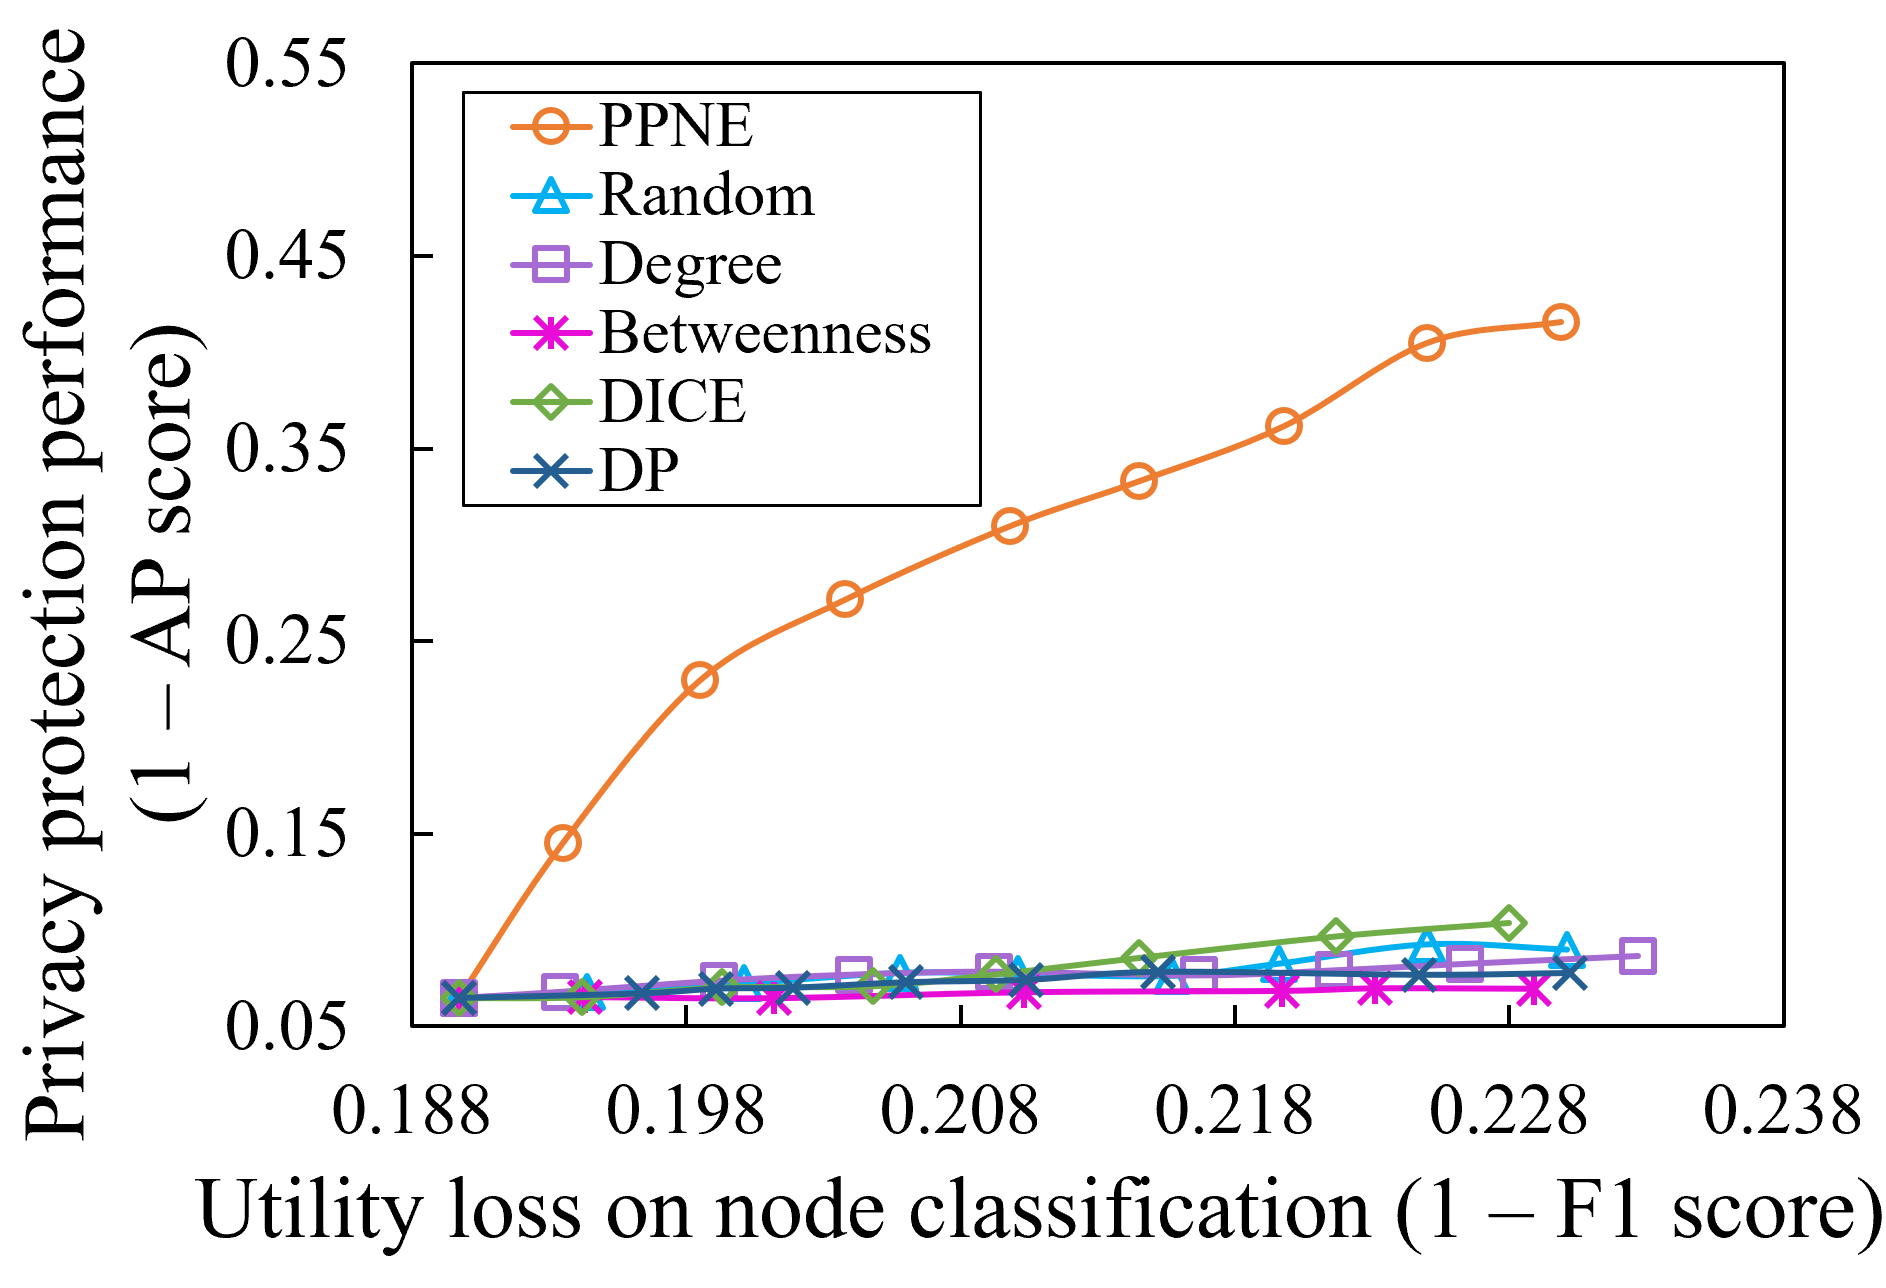}
		\caption{Scenario I on Classification}
		\label{fig:PubDWSINC}
	\end{subfigure}
	\quad %add desired spacing between images, e. g. ~, \quad, \qquad, \hfill etc.
	%(or a blank line to force the subfigure onto a new line)
	\begin{subfigure}[b]{0.23\textwidth}
		\includegraphics[width=\textwidth]{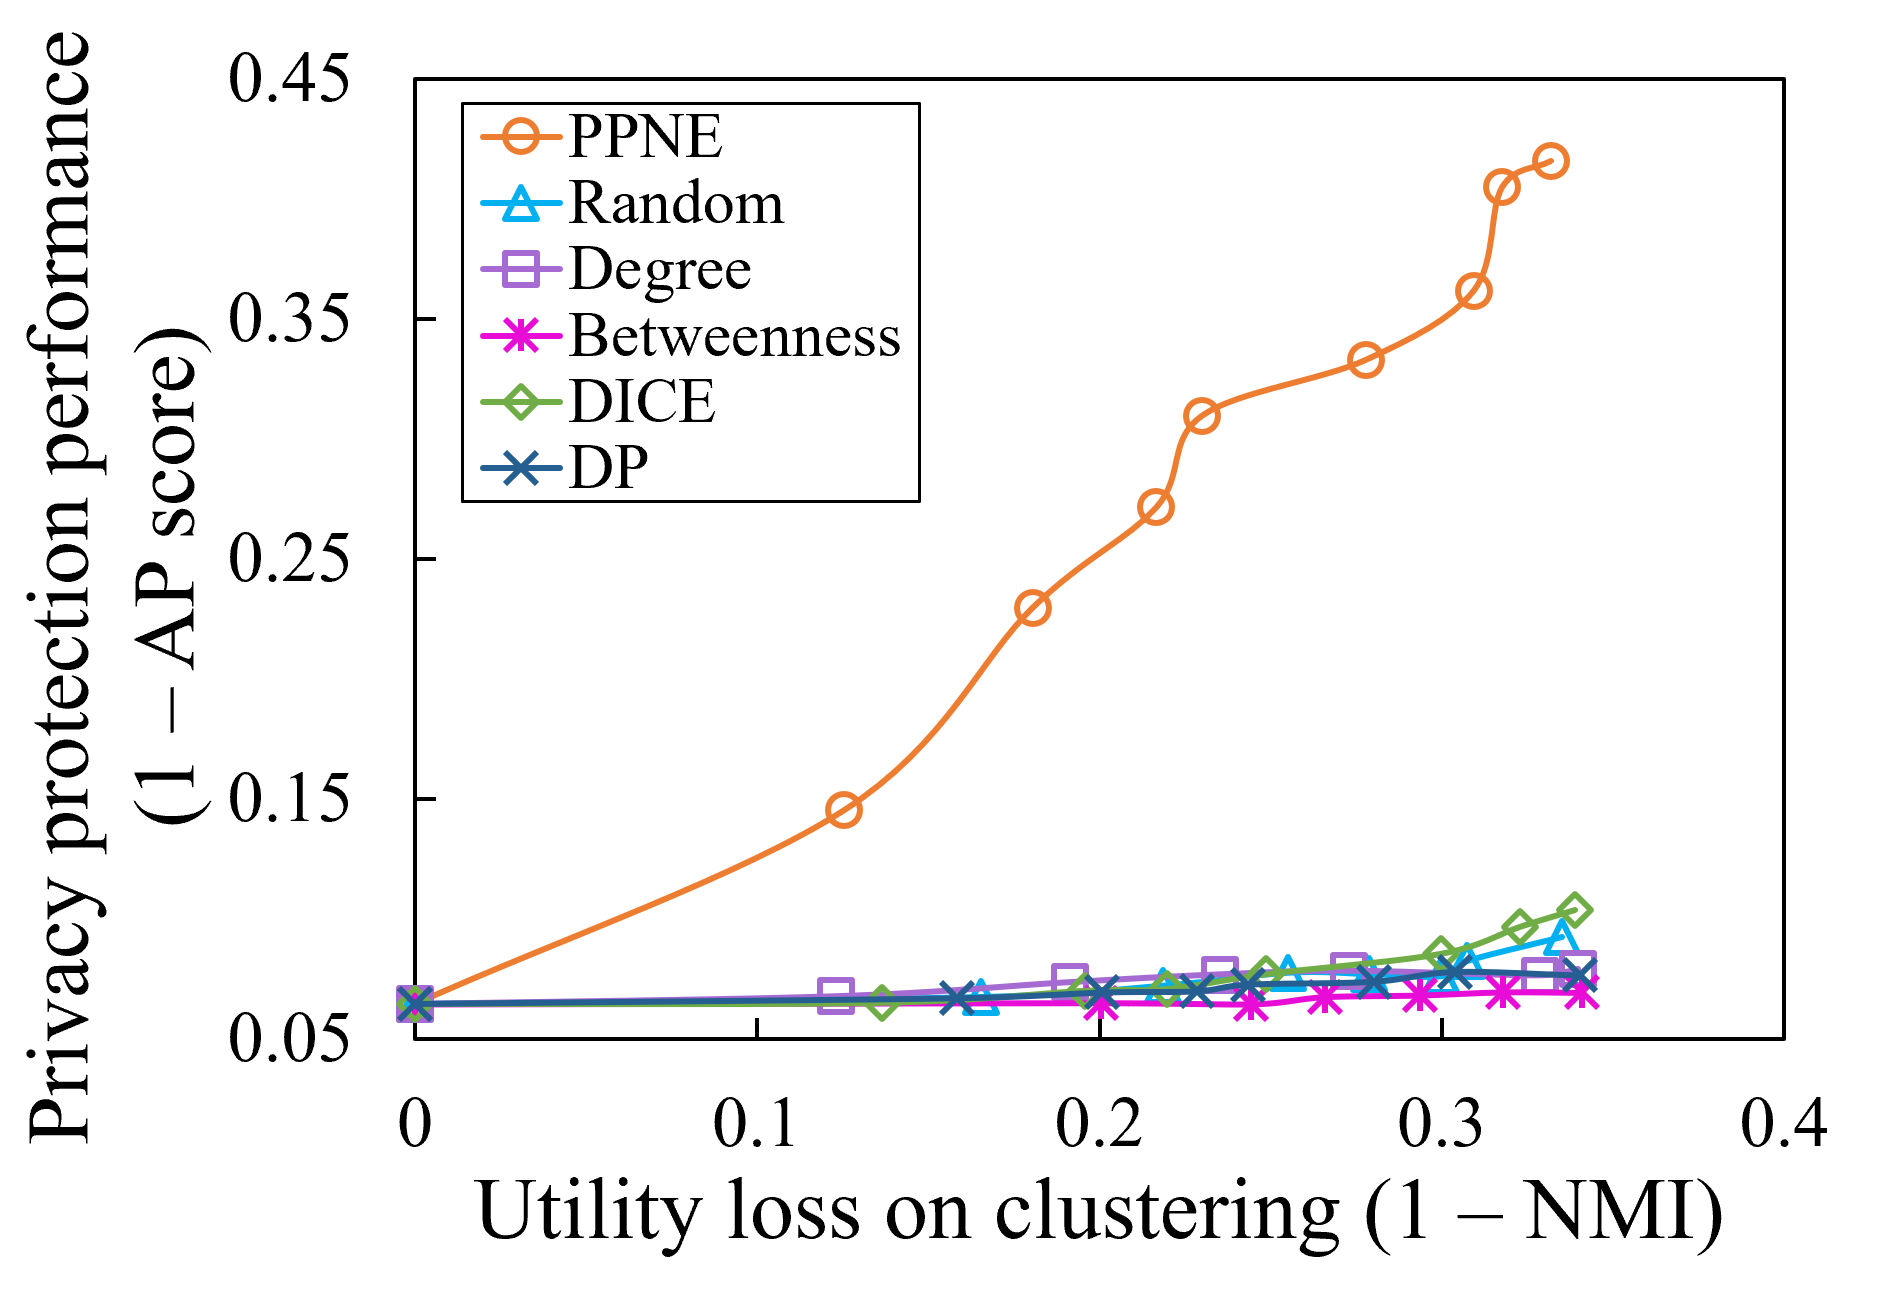}
		\caption{Scenario I on Clustering}
		\label{fig:PubDWSICL}
	\end{subfigure}
	\quad %add desired spacing between images, e. g. ~, \quad, \qquad, \hfill etc.
	%(or a blank line to force the subfigure onto a new line)
	\begin{subfigure}[b]{0.23\textwidth}
		\includegraphics[width=\textwidth]{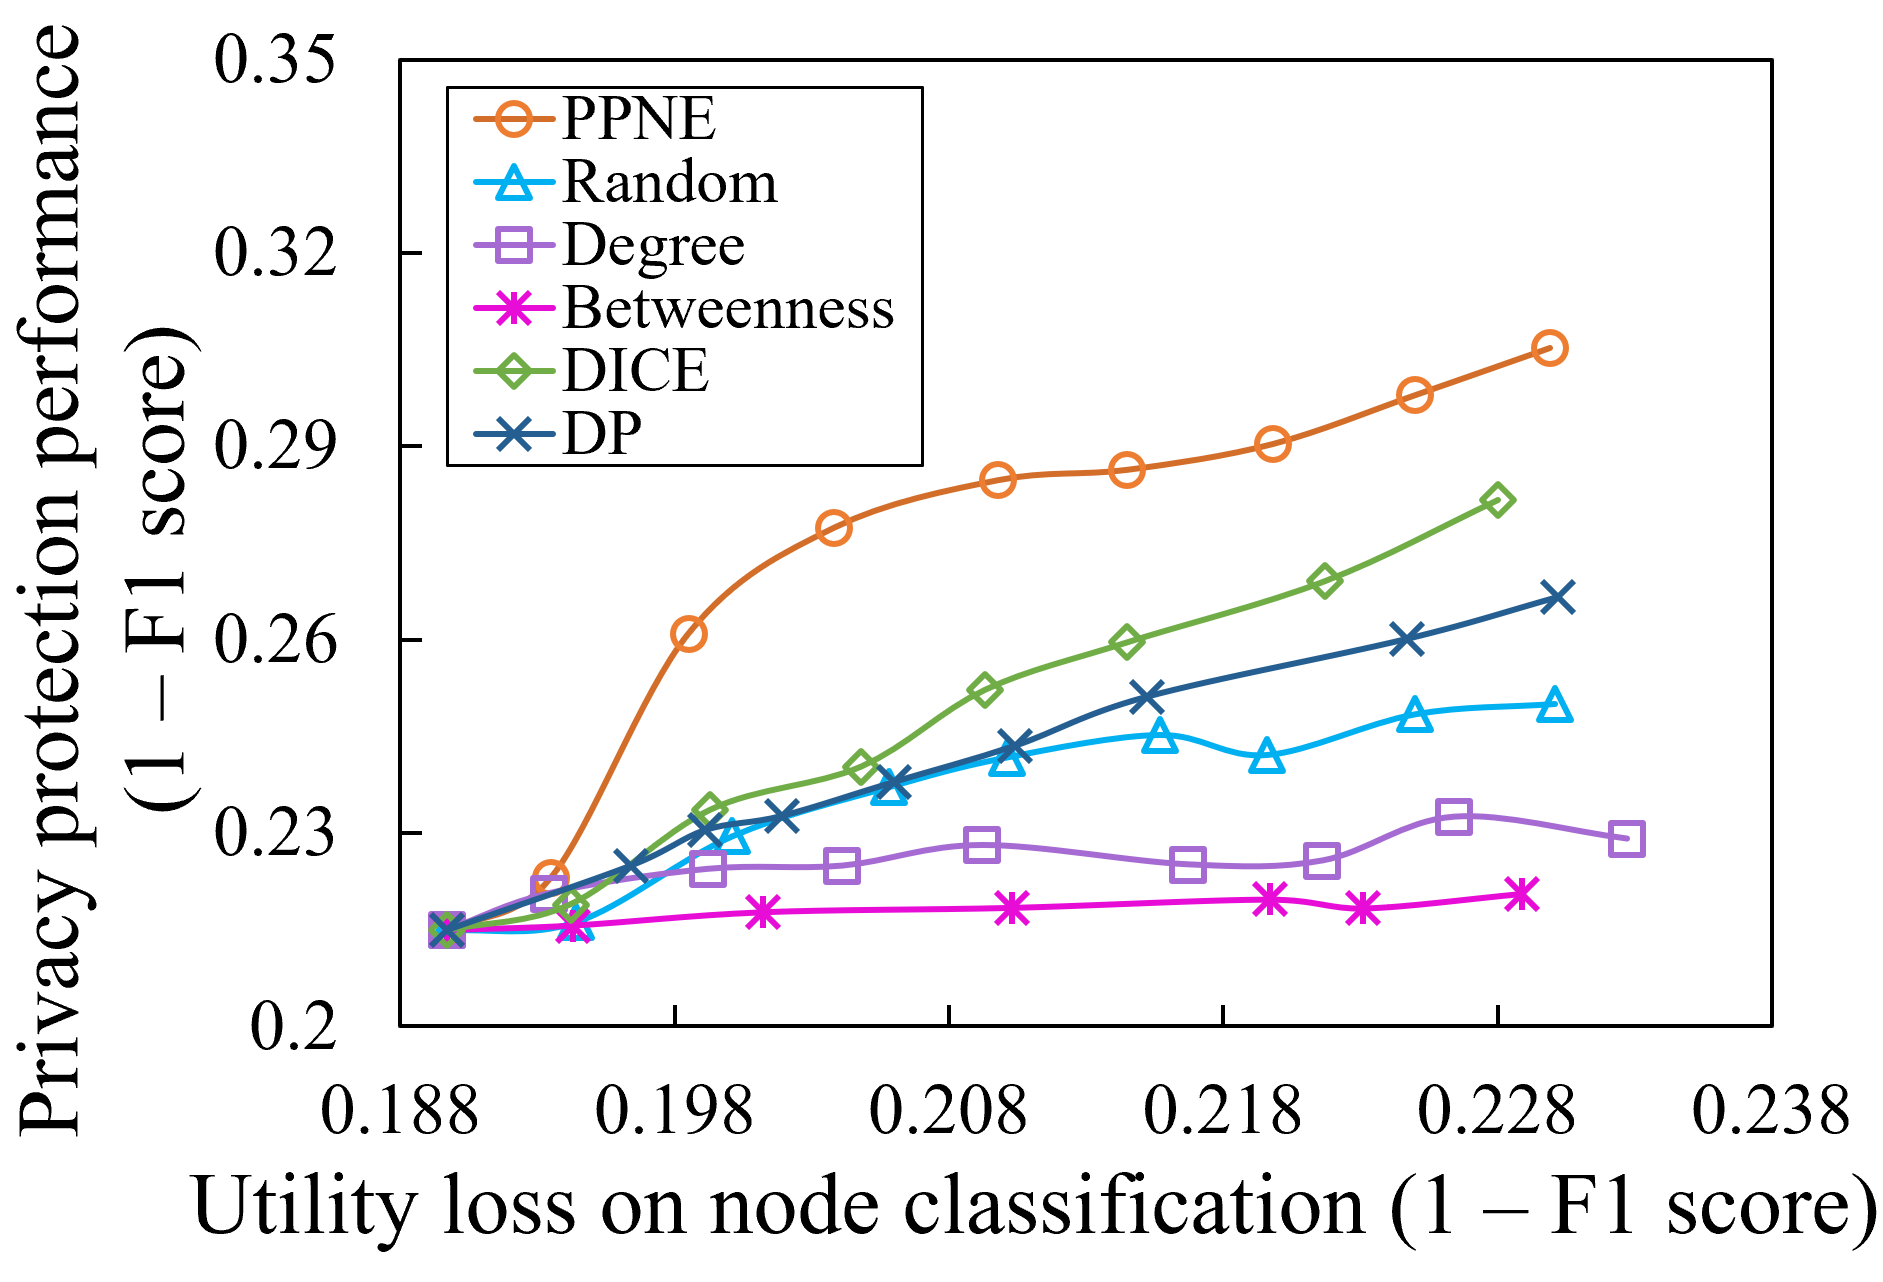}
		\caption{Scenario II on Classification}
		\label{fig:PubDWSIINC}
	\end{subfigure}
	\quad
	\begin{subfigure}[b]{0.23\textwidth}
		\includegraphics[width=\textwidth]{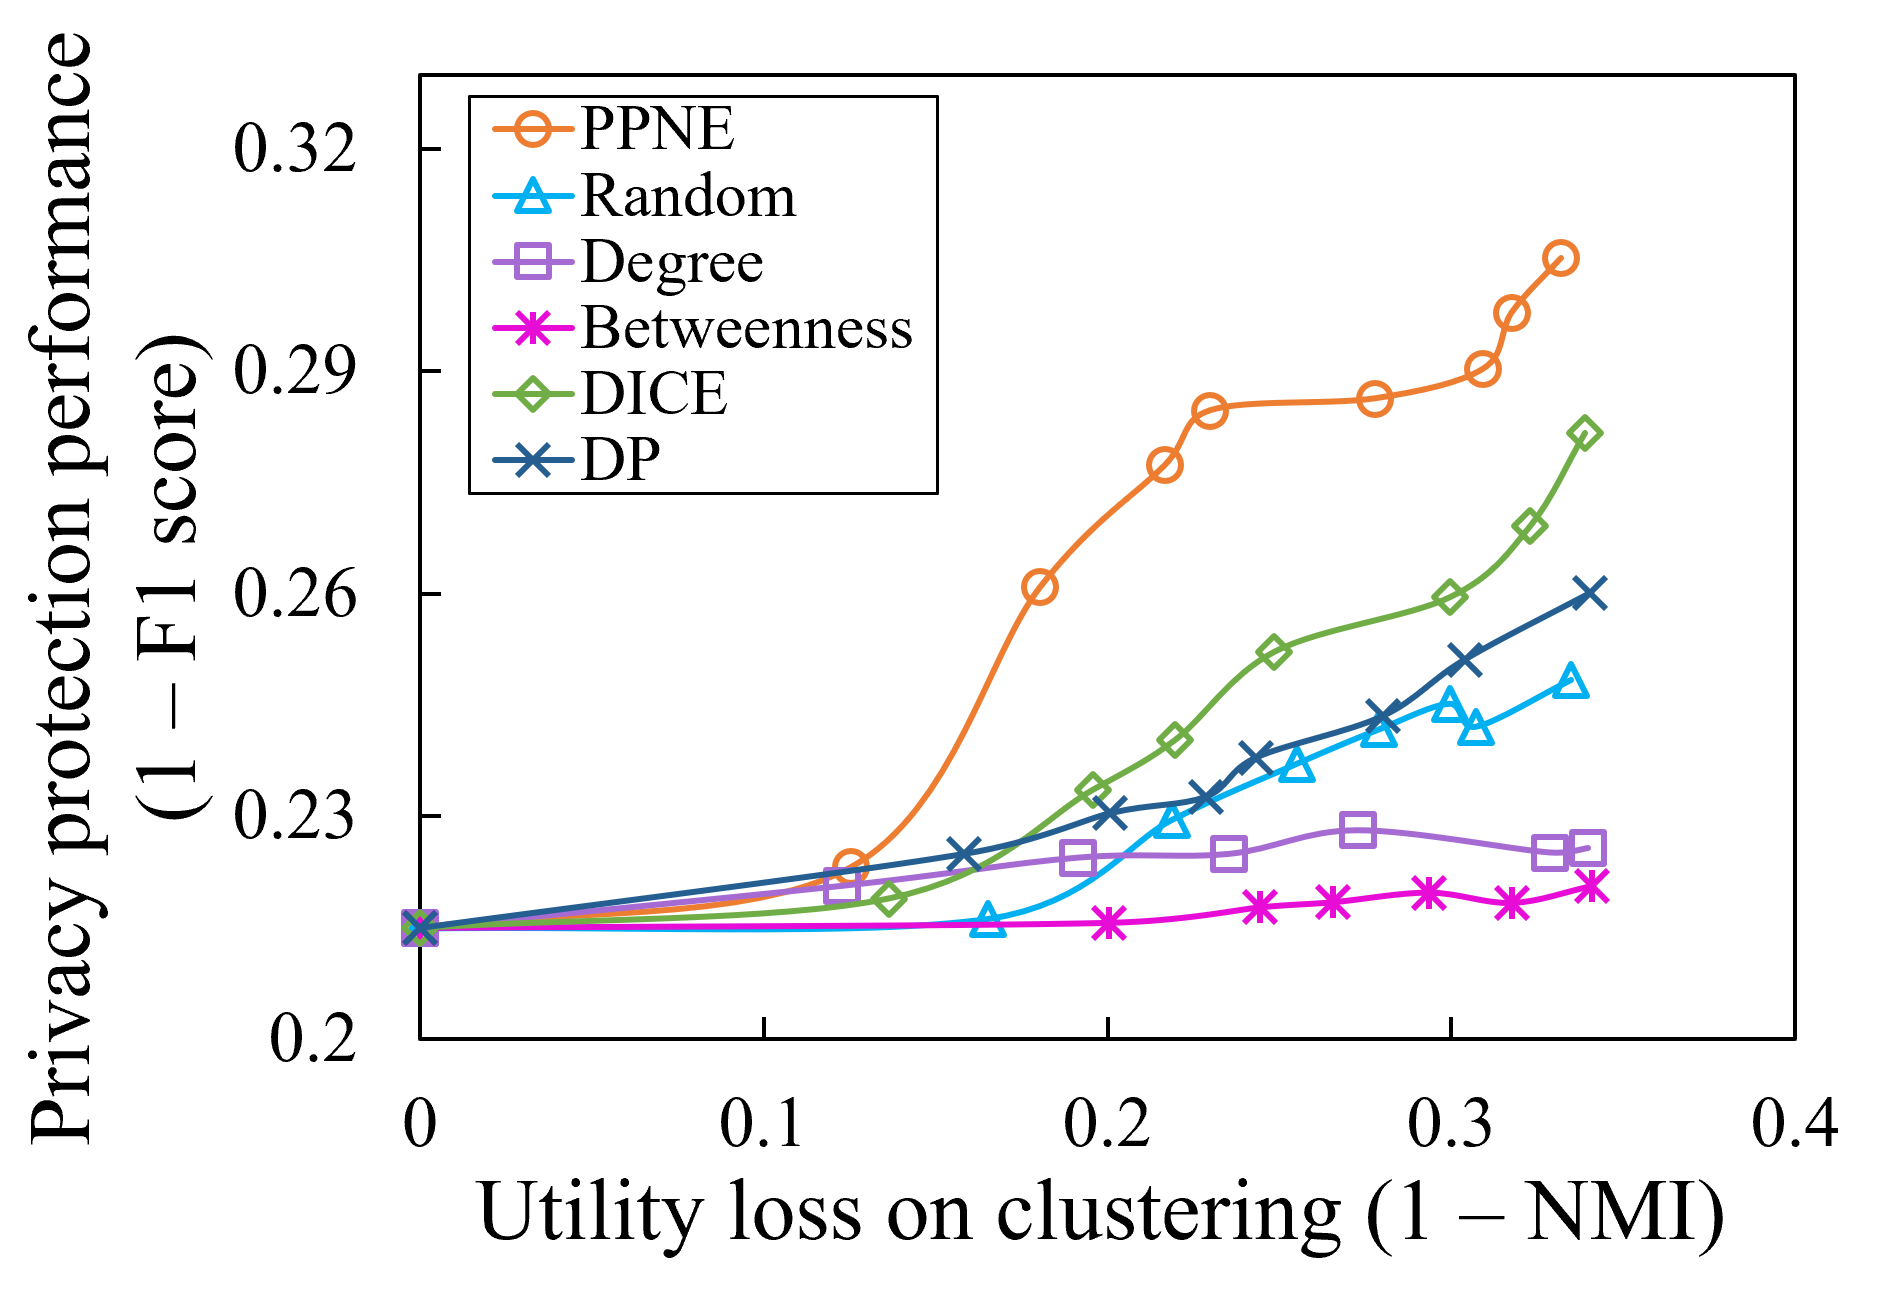}
		\caption{Scenario II on Clustering}
		\label{fig:PubDWSIICL}
	\end{subfigure}
	\vspace{-1em}
	\caption{Tradeoff on PubMed: privacy protection on private links and node classification/clustering performance (DeepWalk)}\label{fig:PubTradeOffDW}
	\vspace{-1em}
\end{figure*}

\begin{figure*}[t]
	\centering
	\begin{subfigure}[b]{0.23\textwidth}
		\includegraphics[width=\textwidth]{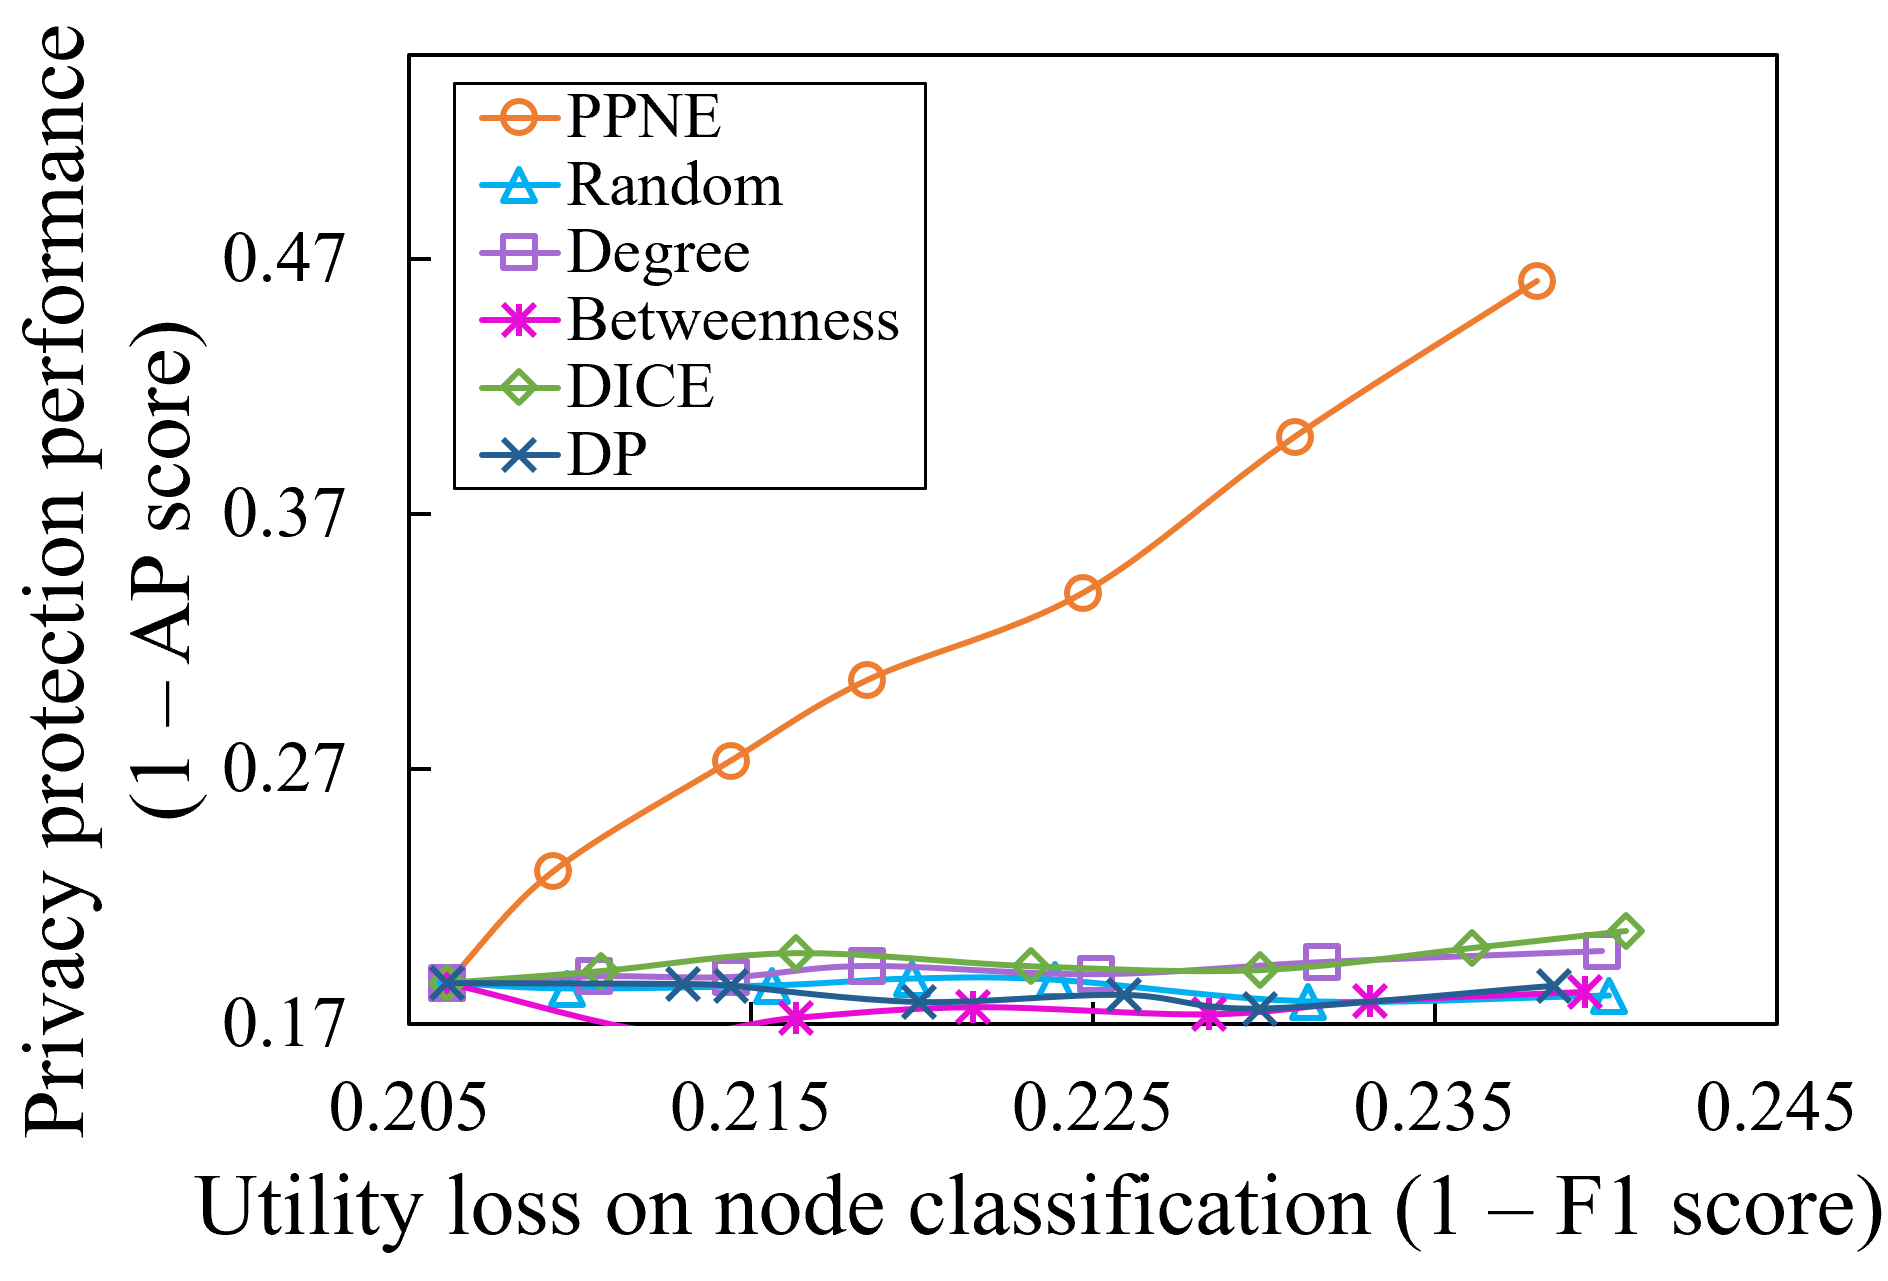}
		\caption{Scenario I on Classification}
		\label{fig:PubLINESINC}
	\end{subfigure}
	\quad %add desired spacing between images, e. g. ~, \quad, \qquad, \hfill etc.
	%(or a blank line to force the subfigure onto a new line)
	\begin{subfigure}[b]{0.23\textwidth}
		\includegraphics[width=\textwidth]{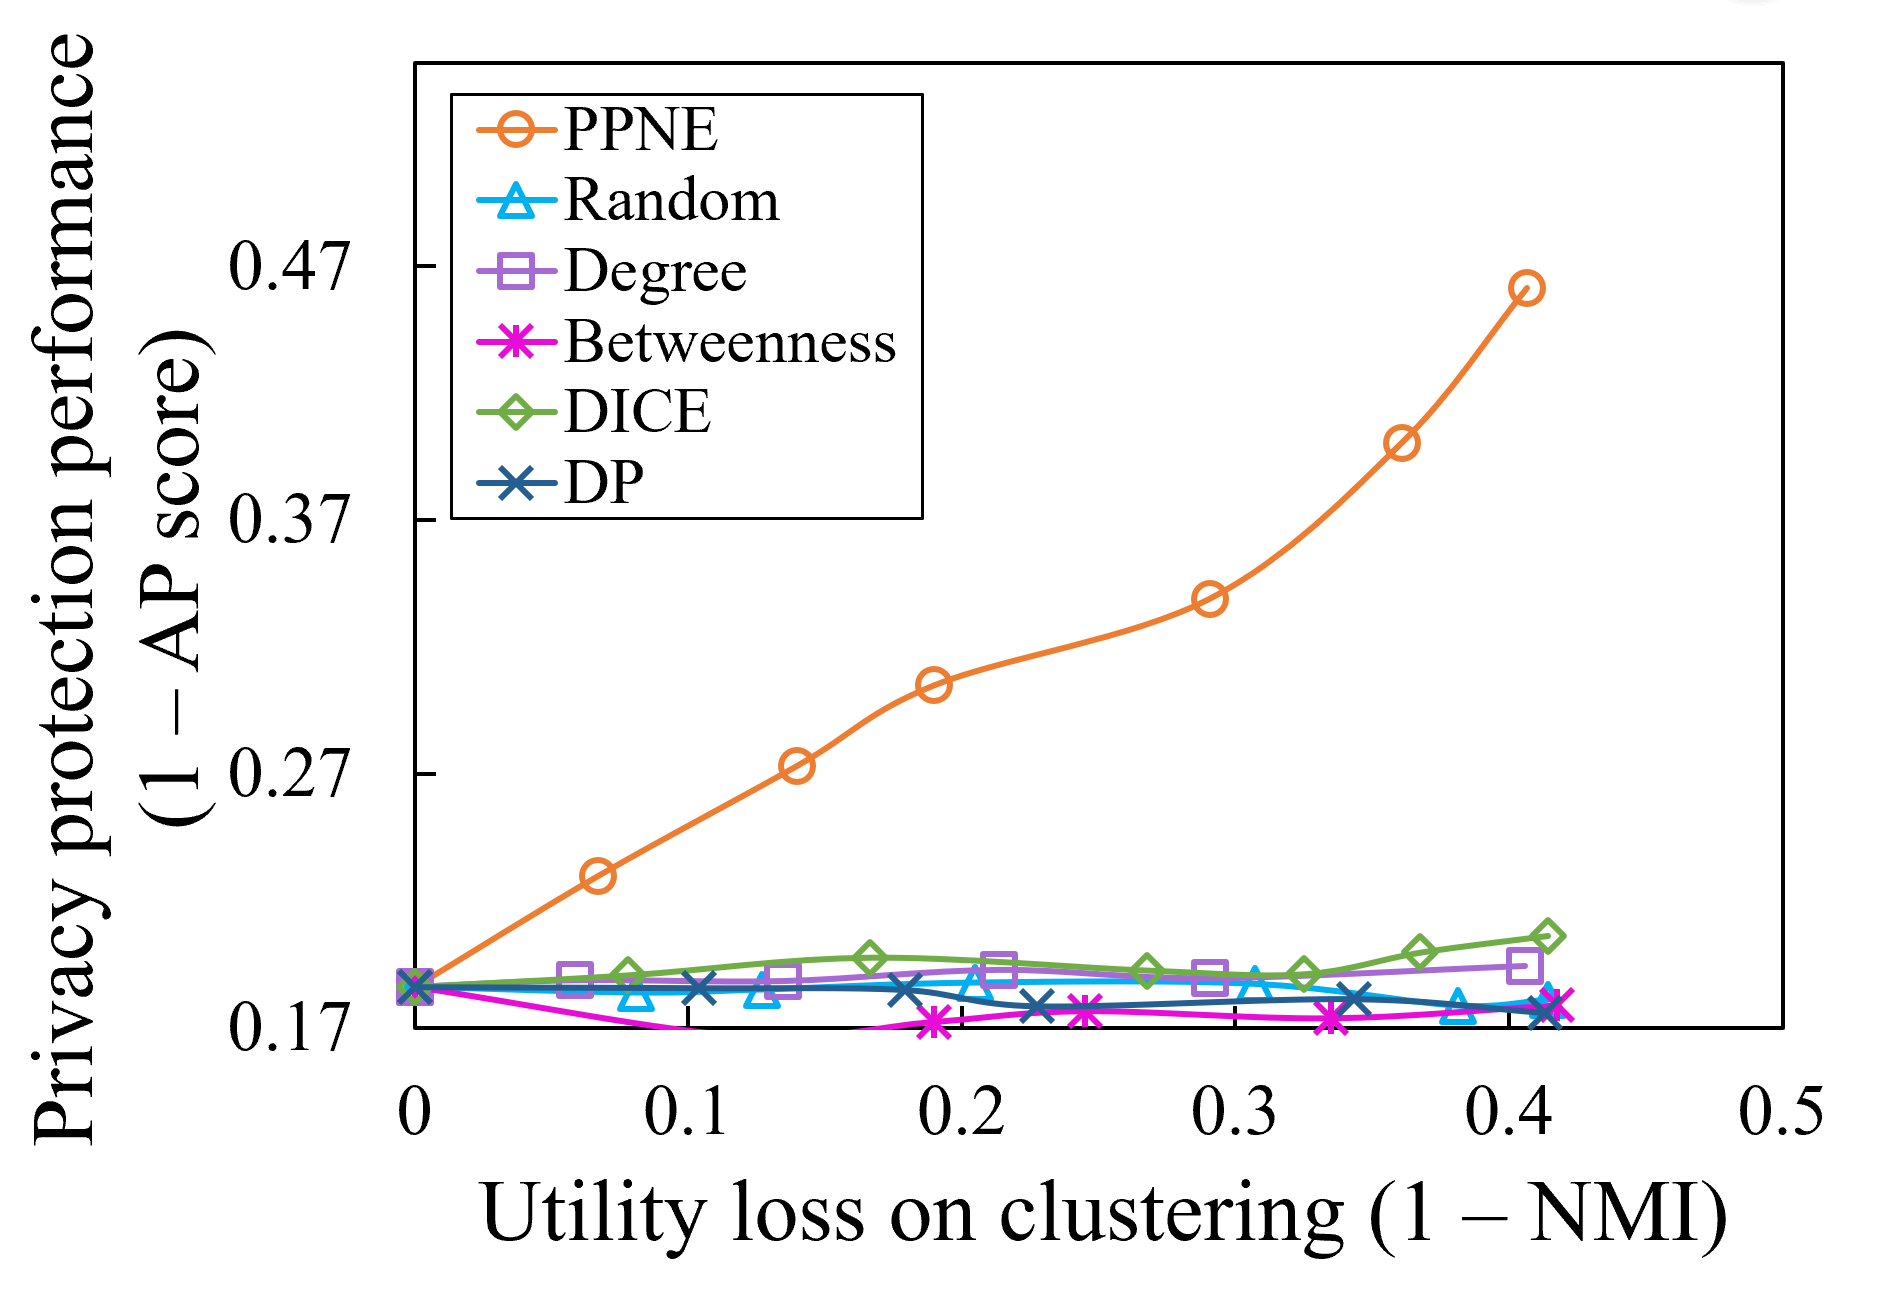}
		\caption{Scenario I on Clustering}
		\label{fig:PubLINESICL}
	\end{subfigure}
	\quad %add desired spacing between images, e. g. ~, \quad, \qquad, \hfill etc.
	%(or a blank line to force the subfigure onto a new line)
	\begin{subfigure}[b]{0.23\textwidth}
		\includegraphics[width=\textwidth]{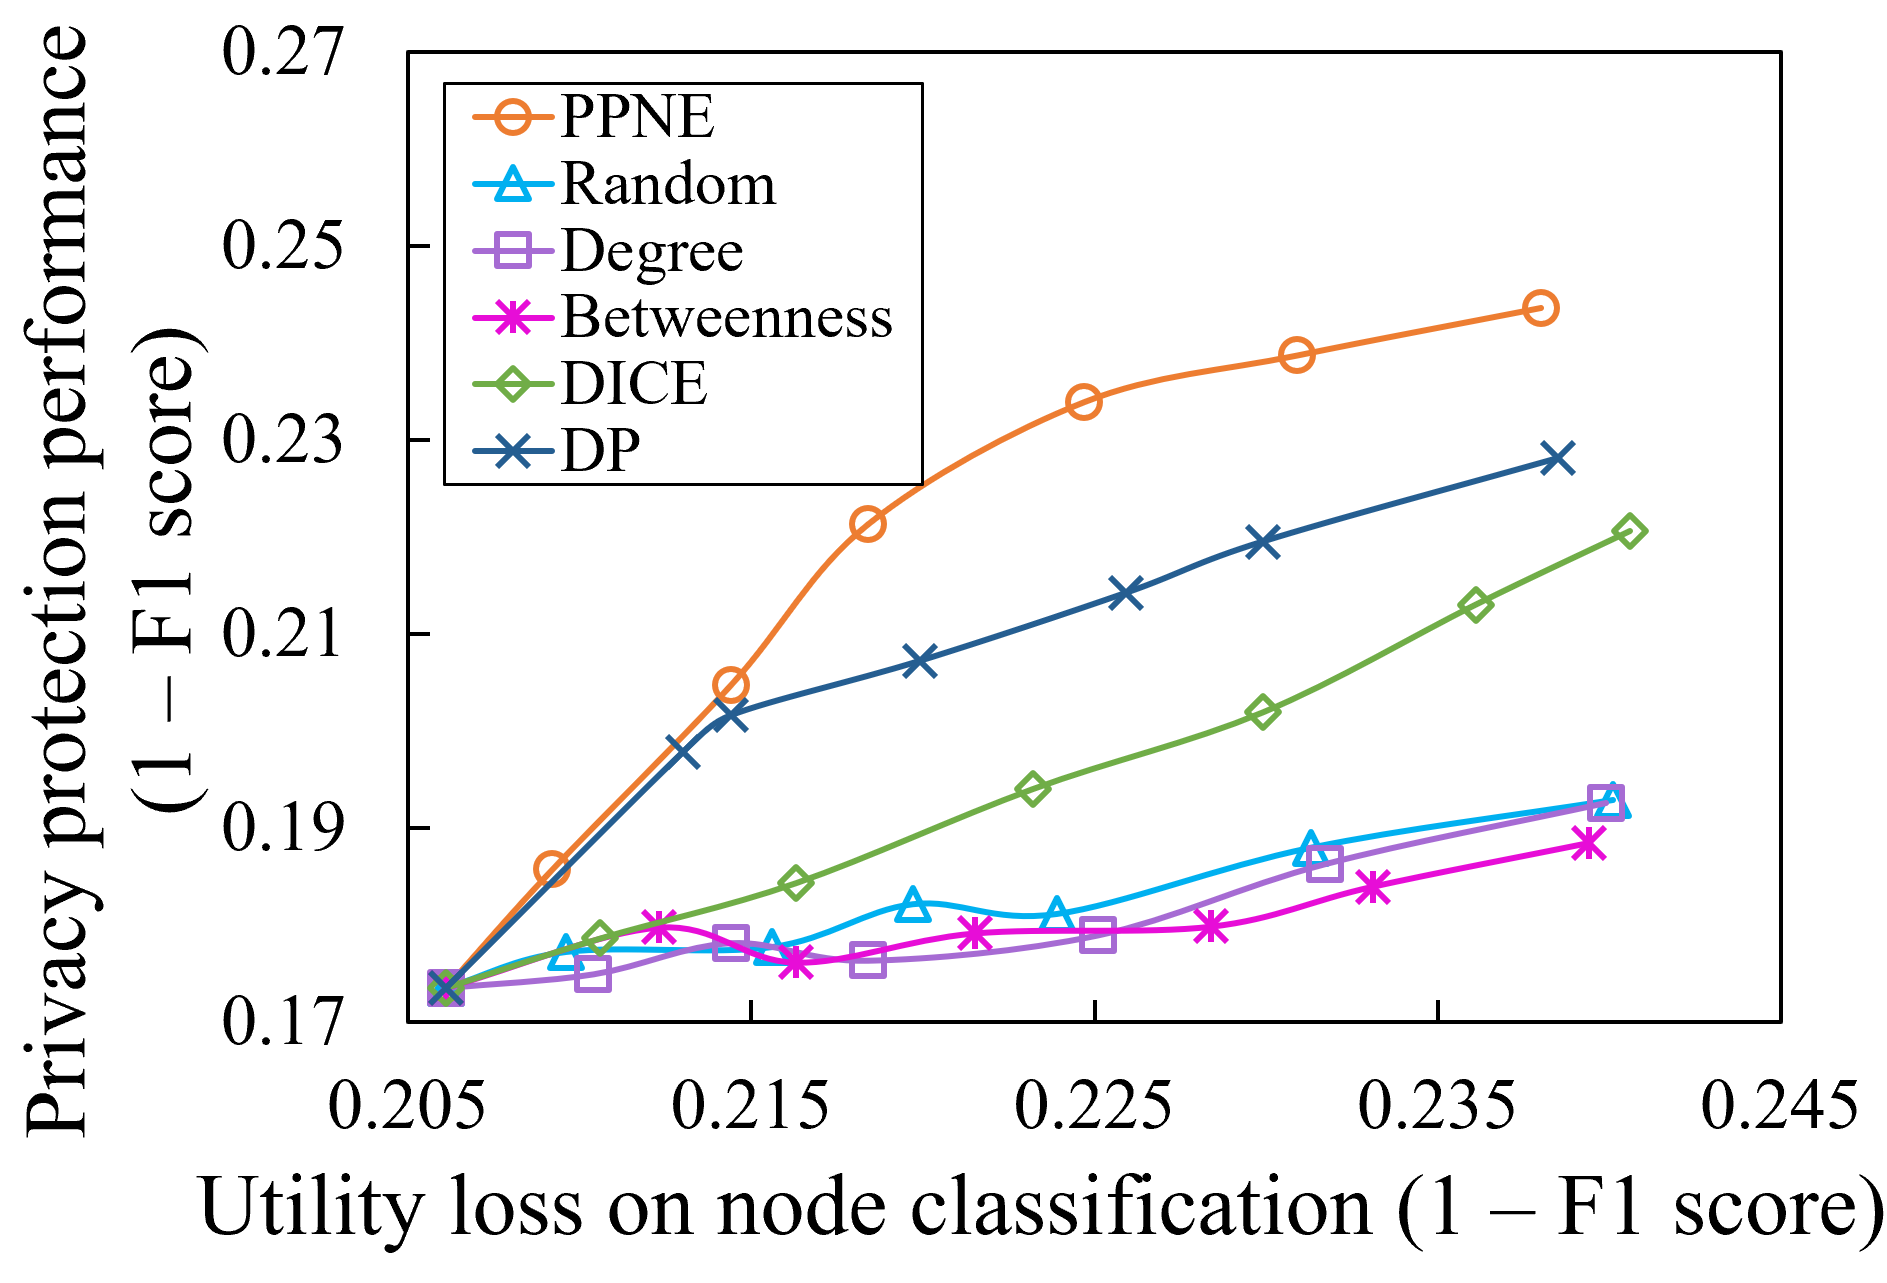}
		\caption{Scenario II on Classification}
		\label{fig:PubLINESIINC}
	\end{subfigure}
	\quad
	\begin{subfigure}[b]{0.23\textwidth}
		\includegraphics[width=\textwidth]{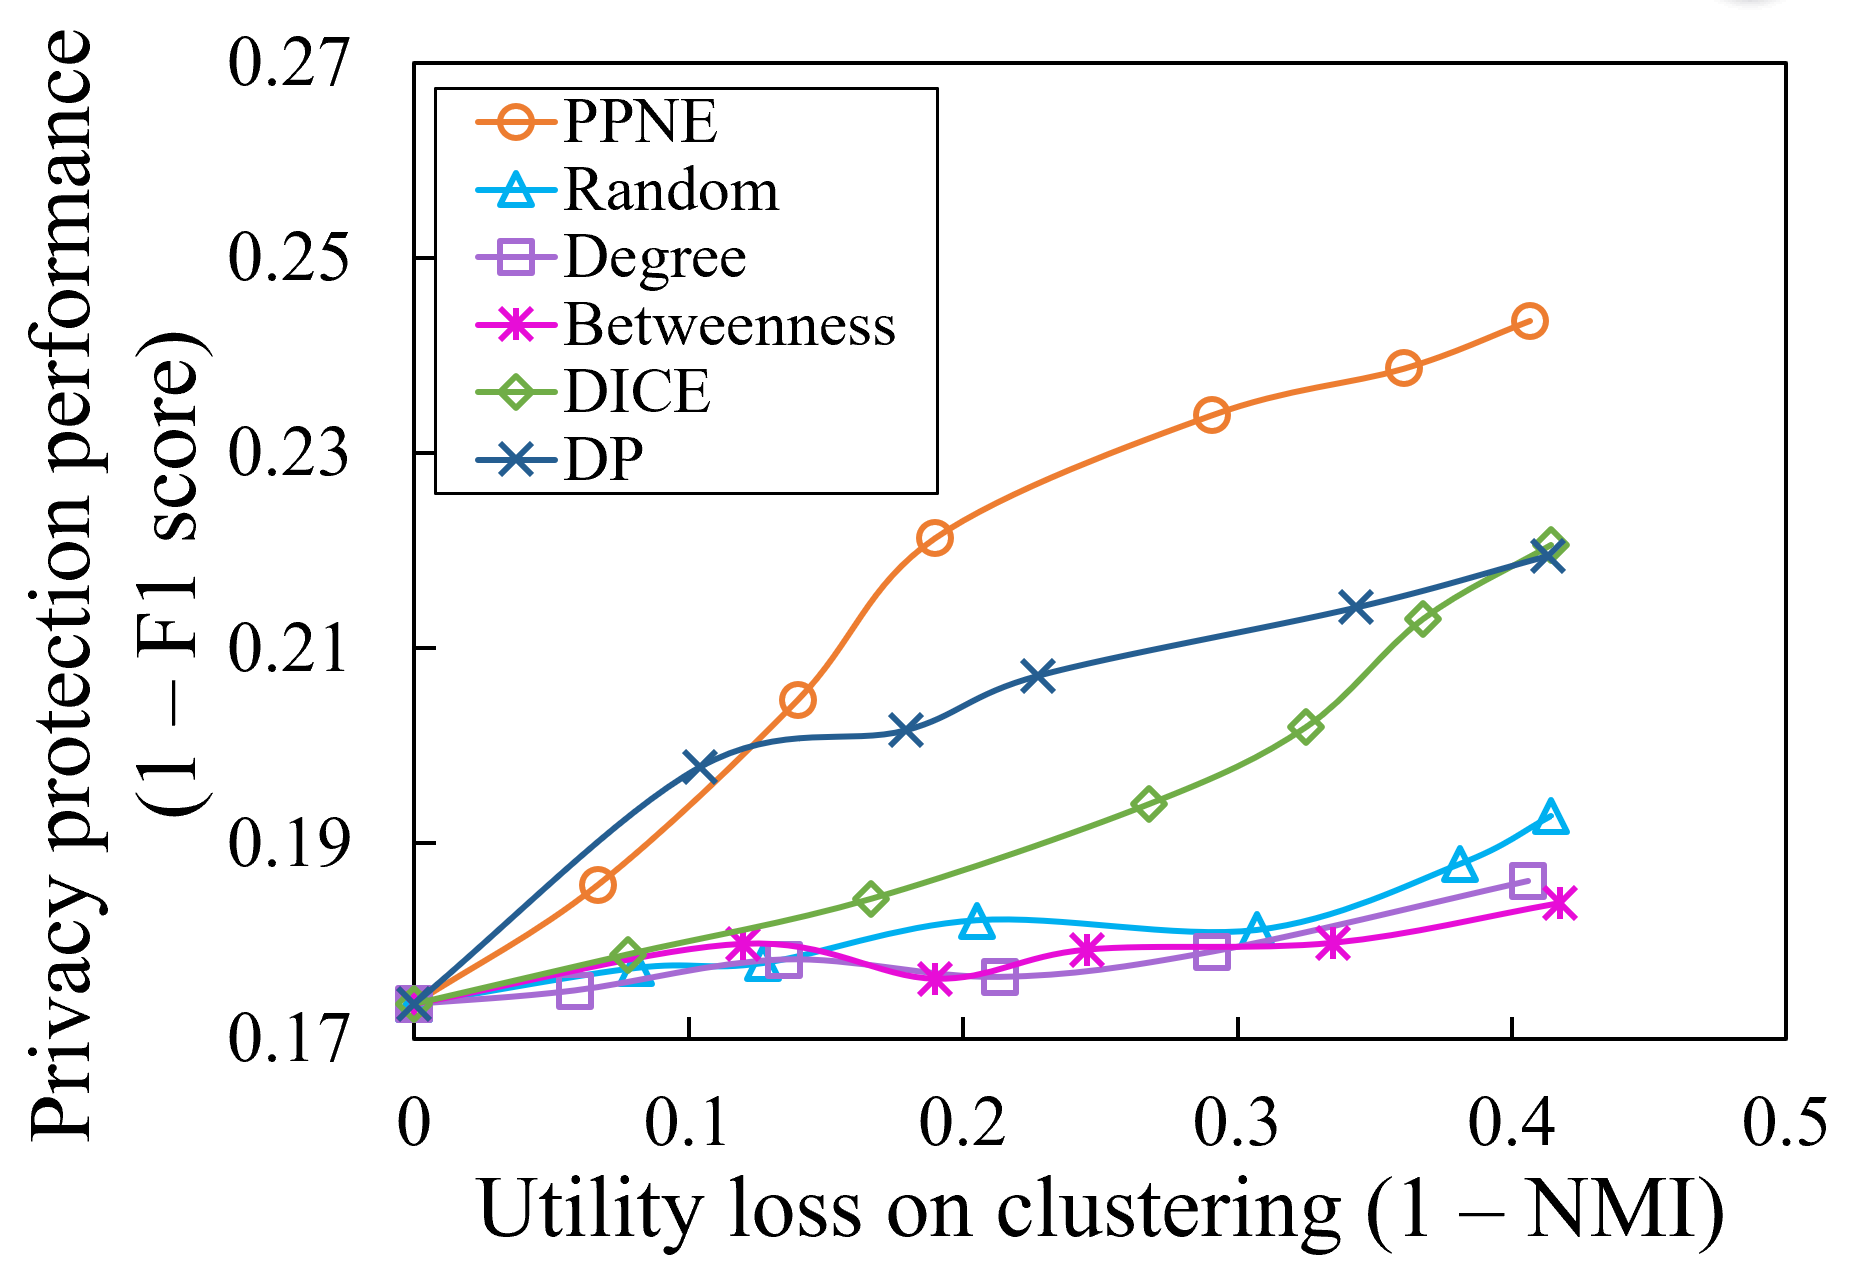}
		\caption{Scenario II on Clustering}
		\label{fig:PubLINESIICL}
	\end{subfigure}
	\vspace{-1em}
	\caption{Tradeoff on PubMed: privacy protection on private links and node classification/clustering performance (LINE)}
	\label{fig:PubTradeOffLINE}
	\vspace{-1em}
\end{figure*}
\subsection{Part Two}

Etiam commodo feugiat nisl pulvinar pellentesque. Etiam auctor sodales
ligula, non varius nibh pulvinar semper. Suspendisse nec lectus non
ipsum convallis congue hendrerit vitae sapien. Donec at laoreet
eros. Vivamus non purus placerat, scelerisque diam eu, cursus
ante. Etiam aliquam tortor auctor efficitur mattis.
